# Supplementary material for: Comprehensive calculations of energy levels, radiative transition parameters, hyperfine structure constants A$_J$-B$_J$, Land\'e g$_J$ factors and isotope shifts for Sc XX
Source: arXiv:2202.03112 source file (2022-02-07)
Supplement: Supplementary file 1 [file Table4.tex]

\documentclass[10pt]{article}
\usepackage{booktabs}
\usepackage{longtable}
\usepackage{subfloat}
\usepackage{bm}
\textwidth = 15 truecm
\textheight = 24 truecm
\hoffset = -2 truecm
\voffset = -2 truecm

\begin{document}
\caption{Table 4. Present radiative parameters for magnetic dipole  M1 transitions and their comparison with the results from Si et al. [32] and the NIST database [41].}
\begin{longtable}{lllllllll}
\toprule
 Upper level & Lower level & A(s$^{-1}$) &    A(s$^{-1}$) [32]   &  A(s$^{-1}$) [NIST]& Our f & f [32] \\
\midrule
$1s\,6s ~^3S_{1}$ &  $1s^2 ~^1S _{0}$&  1.766E+05 &           &          &  4.005E-10 &            &   \\
$1s\,5s ~^3S_{1}$ &  $1s^2 ~^1S _{0}$&  6.586E+05 &           &          &  1.531E-09 &            &   \\
$1s\,4d ~^3D_{1}$ &  $1s^2 ~^1S _{0}$&  6.390E+04 &           &          &  1.553E-10 &            &   \\
$1s\,4s ~^3S_{1}$ &  $1s^2 ~^1S _{0}$&  2.200E+06 &           &          &  5.355E-09 &            &   \\
$1s\,3d ~^3D_{1}$ &  $1s^2 ~^1S _{0}$&  1.024E+05 &           &          &  2.754E-10 &            &   \\
$1s\,3s ~^3S_{1}$ &  $1s^2 ~^1S _{0}$&  7.002E+06 &           &          &  1.893E-08 &            &   \\
$1s\,2s ~^3S_{1}$ &  $1s^2 ~^1S _{0}$&  2.024E+07 &  2.317E+07 &  2.400E+07 &  7.672E-08 &  8.783E-08 &   \\
$1s\,8p ~^1P_{1}$ &  $1s\,2p ~^3P _{0}$&  3.441E+03 &           &          &  1.416E-10 &            &   \\
$1s\,8p ~^3P_{2}$ &  $1s\,2p ~^3P_{1}$ &  7.021E+03 &           &          &  1.608E-10 &            &   \\
$1s\,8s ~^3S_{1}$ &  $1s\,2s ~^1S _{0}$&  2.755E+04 &           &          &  1.138E-09 &            &   \\
$1s\,8p ~^3P_{2}$ &  $1s\,2p ~^1P_{1}$&  6.220E+03 &           &          &  1.472E-10 &            &   \\
$1s\,7p ~^1P_{1}$ &  $1s\,2p ~^3P _{0}$&  2.733E+03 &           &          &  1.171E-10 &            &   \\
$1s\,7p ~^3P_{2}$ &  $1s\,2p ~^3P_{1}$&  1.522E+04 &           &          &  3.633E-10 &            &   \\
$1s\,7s ~^3S_{1}$ &  $1s\,2s ~^1S _{0}$&  1.853E+04 &           &          &  7.977E-10 &            &   \\
$1s\,7p ~^1P_{1}$ &  $1s\,2p ~^3P_{2}$&  4.235E+04 &           &          &  3.668E-10 &            &   \\
$1s\,6p ~^3P_{1}$ &  $1s\,2p ~^3P _{0}$&  8.802E+03 &           &          &  4.026E-10 &            &   \\
$1s\,6p ~^3P_{2}$ &  $1s\,2p ~^3P_{1}$&  3.154E+04 &           &          &   8.03E-10 &            &   \\
$1s\,6s ~^3S_{1}$ &  $1s\,2s ~^1S _{0}$&  1.027E+04 &           &          &  4.719E-10 &            &   \\
$1s\,6p ~^1P_{1}$ &  $1s\,2p ~^3P_{2}$&  1.171E+05 &           &          &  1.082E-09 &            &   \\
$1s\,6p ~^3P_{2}$ &  $1s\,2p ~^1P_{1}$&  1.537E+04 &           &          &  4.047E-10 &            &   \\
$1s\,6p ~^3P _{0}$ &  $1s\,2p ~^1P_{1}$&  1.995E+04 &           &          &  1.051E-10 &            &   \\
$1s\,5p ~^3P_{1}$ &  $1s\,2p ~^3P _{0}$&  4.004E+04 &           &          &  2.049E-09 &            &   \\
$1s\,5p ~^3P_{2}$ &  $1s\,2p ~^3P_{1}$&  5.618E+04 &           &          &  1.599E-09 &            &   \\
$1s\,5p ~^3P _{0}$ &  $1s\,2p ~^3P_{1}$&  5.877E+04 &           &          &   3.35E-10 &            &   \\
$1s\,5p ~^1P_{1}$ &  $1s\,2p ~^3P_{2}$&  2.184E+05 &           &          &  2.258E-09 &            &   \\
$1s\,5p ~^3P_{2}$ &  $1s\,2p ~^1P_{1}$&  3.666E+04 &           &          &  1.082E-09 &            &   \\
$1s\,5p ~^3P _{0}$ &  $1s\,2p ~^1P_{1}$&  8.210E+04 &           &          &   4.85E-10 &            &   \\
$1s\,4s ~^1S _{0}$ &  $1s\,2s ~^3S_{1}$&  6.745E+04 &           &          &  4.603E-10 &            &   \\
$1s\,4p ~^3P_{1}$ &  $1s\,2p ~^3P _{0}$&  7.882E+04 &           &          &  5.053E-09 &            &   \\
$1s\,4p ~^3P_{2}$ &  $1s\,2p ~^3P_{1}$&  1.183E+05 &           &          &  4.217E-09 &            &   \\
$1s\,4p ~^3P _{0}$ &  $1s\,2p ~^3P_{1}$&  1.215E+05 &           &          &  8.673E-10 &            &   \\
$1s\,4p ~^1P_{1}$ &  $1s\,2p ~^3P_{2}$&  5.057E+05 &           &          &  6.538E-09 &            &   \\
$1s\,4s ~^3S_{1}$ &  $1s\,2s ~^1S _{0}$&  6.802E+03 &           &          &    4.4E-10 &            &   \\
$1s\,4p ~^3P_{2}$ &  $1s\,2p ~^1P_{1}$&  1.227E+05 &           &          &  4.553E-09 &            &   \\
$1s\,4p ~^3P _{0}$ &  $1s\,2p ~^1P_{1}$&  1.542E+05 &           &          &  1.146E-09 &            &   \\
$1s\,3s ~^1S _{0}$ &  $1s\,2s ~^3S_{1}$&  2.830E+05 &           &          &   3.46E-09 &            &   \\
$1s\,3p ~^1P_{1}$ &  $1s\,2p ~^3P _{0}$&  4.144E+03 &           &          &  4.755E-10 &            &   \\
$1s\,3p ~^3P_{2}$ &  $1s\,2p ~^3P_{1}$&  2.750E+05 &           &          &  1.777E-08 &            &   \\
$1s\,3p ~^3P_{1}$ &  $1s\,2p ~^3P _{0}$&  3.012E+05 &           &          &  3.509E-08 &            &   \\
$1s\,3p ~^1P_{1}$ &  $1s\,2p ~^3P_{2}$&  1.264E+06 &           &          &  2.952E-08 &            &   \\
$1s\,3p ~^3P _{0}$ &  $1s\,2p ~^3P_{1}$&  5.965E+05 &           &          &   7.75E-09 &            &   \\
$1s\,3p ~^3P_{1}$ &  $1s\,2p ~^3P_{2}$&  1.692E+04 &           &          &   4.01E-10 &            &   \\
$1s\,3s ~^3S_{1}$ &  $1s\,2s ~^1S _{0}$&  8.507E+04 &           &          &  1.013E-08 &            &   \\
$1s\,3p ~^3P_{2}$ &  $1s\,2p ~^1P_{1}$&  4.060E+05 &           &          &  2.771E-08 &            &   \\
$1s\,3p ~^3P _{0}$ &  $1s\,2p ~^1P_{1}$&  4.991E+05 &           &          &  6.847E-09 &            &   \\
$1s\,8s ~^1S _{0}$ &  $1s\,3s ~^3S_{1}$&  4.413E+03 &           &          &  1.198E-10 &            &   \\
$1s\,8p ~^1P_{1}$ &  $1s\,3p ~^3P _{0}$&  2.216E+03 &           &          &  5.534E-10 &            &   \\
$1s\,8p ~^3P_{1}$ &  $1s\,3p ~^3P _{0}$&  2.134E+04 &           &          &  5.334E-09 &            &   \\
$1s\,8p ~^3P _{0}$ &  $1s\,3p ~^3P_{1}$&  5.289E+04 &           &          &  1.471E-09 &            &   \\
$1s\,8d ~^1D_{2}$ &  $1s\,3d ~^3D_{1}$&  1.977E+03 &           &          &    2.8E-10 &            &   \\
$1s\,8d ~^3D_{1}$ &  $1s\,3d ~^3D_{2}$&  9.436E+04 &           &          &  4.812E-09 &            &   \\
$1s\,8d ~^3D_{2}$ &  $1s\,3d ~^3D_{1}$&  5.581E+04 &           &          &  7.903E-09 &            &   \\
$1s\,8d ~^1D_{2}$ &  $1s\,3d ~^3D_{3}$&  4.678E+04 &           &          &  2.846E-09 &            &   \\
$1s\,8d ~^3D_{2}$ &  $1s\,3d ~^3D_{3}$&  2.242E+03 &           &          &  1.364E-10 &            &   \\
$1s\,8d ~^3D_{3}$ &  $1s\,3d ~^1D_{2}$&  3.497E+04 &           &          &  4.174E-09 &            &   \\
$1s\,8p ~^3P_{2}$ &  $1s\,3p ~^1P_{1}$&  3.083E+03 &           &          &   4.38E-10 &            &   \\
$1s\,8p ~^3P _{0}$ &  $1s\,3p ~^1P_{1}$&  1.311E+04 &           &          &  3.727E-10 &            &   \\
$1s\,7s ~^1S _{0}$ &  $1s\,3s ~^3S_{1}$&  1.147E+04 &           &          &  3.443E-10 &            &   \\
$1s\,7p ~^1P_{1}$ &  $1s\,3p ~^3P _{0}$&  4.000E+03 &           &          &  1.106E-09 &            &   \\
$1s\,7p ~^3P_{1}$ &  $1s\,3p ~^3P _{0}$&  3.742E+04 &           &          &  1.036E-08 &            &   \\
$1s\,7p ~^3P_{2}$ &  $1s\,3p ~^3P_{1}$&  7.231E+02 &           &          &  1.113E-10 &            &   \\
$1s\,7p ~^3P _{0}$ &  $1s\,3p ~^3P_{1}$&  9.537E+04 &           &          &  2.939E-09 &            &   \\
$1s\,7s ~^3S_{1}$ &  $1s\,3s ~^1S _{0}$&  7.289E+02 &           &          &  2.024E-10 &            &   \\
$1s\,7d ~^1D_{2}$ &  $1s\,3d ~^3D_{1}$&  2.114E+03 &           &          &  3.318E-10 &            &   \\
$1s\,7d ~^3D_{1}$ &  $1s\,3d ~^3D_{2}$&  1.002E+05 &           &          &  5.662E-09 &            &   \\
$1s\,7d ~^3D_{2}$ &  $1s\,3d ~^3D_{1}$&  5.936E+04 &           &          &   9.32E-09 &            &   \\
$1s\,7d ~^1D_{2}$ &  $1s\,3d ~^3D_{3}$&  4.764E+04 &           &          &  3.211E-09 &            &   \\
$1s\,7d ~^3D_{2}$ &  $1s\,3d ~^3D_{3}$&  2.432E+03 &           &          &   1.64E-10 &            &   \\
$1s\,7d ~^3D_{3}$ &  $1s\,3d ~^1D_{2}$&  3.578E+04 &           &          &  4.732E-09 &            &   \\
$1s\,7p ~^3P_{2}$ &  $1s\,3p ~^1P_{1}$&  8.605E+02 &           &          &  1.356E-10 &            &   \\
$1s\,7p ~^3P _{0}$ &  $1s\,3p ~^1P_{1}$&  2.547E+04 &           &          &  8.033E-10 &            &   \\
$1s\,6s ~^1S _{0}$ &  $1s\,3s ~^3S_{1}$&  2.693E+04 &           &          &   9.55E-10 &            &   \\
$1s\,6p ~^1P_{1}$ &  $1s\,3p ~^3P _{0}$&  7.918E+03 &           &          &  2.588E-09 &            &   \\
$1s\,6p ~^3P_{1}$ &  $1s\,3p ~^3P _{0}$&  7.029E+04 &           &          &  2.304E-08 &            &   \\
$1s\,6p ~^3P_{2}$ &  $1s\,3p ~^3P_{1}$&  1.351E+03 &           &          &  2.461E-10 &            &   \\
$1s\,6p ~^3P _{0}$ &  $1s\,3p ~^3P_{1}$&  1.842E+05 &           &          &   6.72E-09 &            &   \\
$1s\,6s ~^3S_{1}$ &  $1s\,3s ~^1S _{0}$&  3.838E+03 &           &          &  1.264E-09 &            &   \\
$1s\,6d ~^1D_{2}$ &  $1s\,3d ~^3D_{1}$&  2.467E+03 &           &          &  4.587E-10 &            &   \\
$1s\,6d ~^3D_{1}$ &  $1s\,3d ~^3D_{2}$&  1.175E+05 &           &          &  7.864E-09 &            &   \\
$1s\,6d ~^3D_{2}$ &  $1s\,3d ~^3D_{1}$&  6.973E+04 &           &          &  1.297E-08 &            &   \\
$1s\,6d ~^1D_{2}$ &  $1s\,3d ~^3D_{3}$&  6.326E+04 &           &          &  5.054E-09 &            &   \\
$1s\,6d ~^3D_{2}$ &  $1s\,3d ~^3D_{3}$&  3.217E+03 &           &          &  2.571E-10 &            &   \\
$1s\,6d ~^3D_{3}$ &  $1s\,3d ~^1D_{2}$&  4.758E+04 &           &          &  7.456E-09 &            &   \\
$1s\,6p ~^3P _{0}$ &  $1s\,3p ~^1P_{1}$&  5.265E+04 &           &          &   1.97E-09 &            &   \\
$1s\,5s ~^1S _{0}$ &  $1s\,3s ~^3S_{1}$&  6.413E+04 &           &          &  3.105E-09 &            &   \\
$1s\,5p ~^1P_{1}$ &  $1s\,3p ~^3P _{0}$&  1.534E+04 &           &          &  6.854E-09 &            &   \\
$1s\,5p ~^3P_{2}$ &  $1s\,3p ~^3P_{1}$&  7.768E+02 &           &          &   1.94E-10 &            &   \\
$1s\,5p ~^3P_{1}$ &  $1s\,3p ~^3P _{0}$&  1.309E+05 &           &          &  5.884E-08 &            &   \\
$1s\,5p ~^3P _{0}$ &  $1s\,3p ~^3P_{1}$&  3.503E+05 &           &          &  1.754E-08 &            &   \\
$1s\,5s ~^3S_{1}$ &  $1s\,3s ~^1S _{0}$&  1.428E+04 &           &          &  6.473E-09 &            &   \\
$1s\,5p ~^3P_{1}$ &  $1s\,3p ~^3P_{2}$&  4.308E+03 &           &          &  3.912E-10 &            &   \\
$1s\,5d ~^1D_{2}$ &  $1s\,3d ~^3D_{1}$&  3.343E+03 &           &          &  8.527E-10 &            &   \\
$1s\,5d ~^3D_{1}$ &  $1s\,3d ~^3D_{2}$&  1.672E+05 &           &          &  1.537E-08 &            &   \\
$1s\,5d ~^3D_{2}$ &  $1s\,3d ~^3D_{1}$&  9.947E+04 &           &          &   2.54E-08 &            &   \\
$1s\,5d ~^1D_{2}$ &  $1s\,3d ~^3D_{3}$&  9.503E+04 &           &          &  1.042E-08 &            &   \\
$1s\,5d ~^3D_{2}$ &  $1s\,3d ~^3D_{3}$&  4.557E+03 &           &          &  5.003E-10 &            &   \\
$1s\,5d ~^3D_{3}$ &  $1s\,3d ~^1D_{2}$&  7.136E+04 &           &          &  1.536E-08 &            &   \\
$1s\,5p ~^3P_{2}$ &  $1s\,3p ~^1P_{1}$&  2.500E+03 &           &          &  6.433E-10 &            &   \\
$1s\,5p ~^3P _{0}$ &  $1s\,3p ~^1P_{1}$&  1.025E+05 &           &          &  5.287E-09 &            &   \\
$1s\,4s ~^1S _{0}$ &  $1s\,3s ~^3S_{1}$&  1.487E+05 &           &          &  1.516E-08 &            &   \\
$1s\,4p ~^1P_{1}$ &  $1s\,3p ~^3P _{0}$&  2.527E+04 &           &          &  2.382E-08 &            &   \\
$1s\,4p ~^1P_{1}$ &  $1s\,3p ~^3P_{2}$&  6.985E+03 &           &          &  1.337E-09 &            &   \\
$1s\,4p ~^3P_{2}$ &  $1s\,3p ~^3P_{1}$&  3.719E+03 &           &          &  1.977E-09 &            &   \\
$1s\,4p ~^3P_{1}$ &  $1s\,3p ~^3P _{0}$&  2.125E+05 &           &          &   2.04E-07 &            &   \\
$1s\,4p ~^3P _{0}$ &  $1s\,3p ~^3P_{1}$&  5.764E+05 &           &          &  6.167E-08 &            &   \\
$1s\,4p ~^3P_{1}$ &  $1s\,3p ~^3P_{2}$&  1.450E+03 &           &          &  2.826E-10 &            &   \\
$1s\,4d ~^1D_{2}$ &  $1s\,3d ~^3D_{1}$&  6.149E+03 &           &          &   3.35E-09 &            &   \\
$1s\,4s ~^3S_{1}$ &  $1s\,3s ~^1S _{0}$&  4.502E+04 &           &          &  4.418E-08 &            &   \\
$1s\,4d ~^3D_{3}$ &  $1s\,3d ~^3D_{2}$&  6.166E+02 &           &          &  2.824E-10 &            &   \\
$1s\,4d ~^3D_{1}$ &  $1s\,3d ~^3D_{2}$&  3.714E+05 &           &          &  7.306E-08 &            &   \\
$1s\,4d ~^3D_{2}$ &  $1s\,3d ~^3D_{1}$&  2.217E+05 &           &          &  1.212E-07 &            &   \\
$1s\,4d ~^1D_{2}$ &  $1s\,3d ~^3D_{3}$&  1.464E+05 &           &          &  3.436E-08 &            &   \\
$1s\,4d ~^3D_{3}$ &  $1s\,3d ~^1D_{2}$&  1.093E+05 &           &          &  5.038E-08 &            &   \\
$1s\,4d ~^3D_{2}$ &  $1s\,3d ~^3D_{3}$&  6.004E+03 &           &          &  1.413E-09 &            &   \\
$1s\,4d ~^3D_{1}$ &  $1s\,3d ~^1D_{2}$&  1.957E+03 &           &          &  3.874E-10 &            &   \\
$1s\,4p ~^3P_{2}$ &  $1s\,3p ~^1P_{1}$&  2.926E+02 &           &          &  1.625E-10 &            &   \\
$1s\,4p ~^3P _{0}$ &  $1s\,3p ~^1P_{1}$&  1.610E+05 &           &          &  1.799E-08 &            &   \\
$1s\,8s ~^1S _{0}$ &  $1s\,4s ~^3S_{1}$&  9.518E+03 &           &          &   1.08E-09 &            &   \\
$1s\,8p ~^1P_{1}$ &  $1s\,4p ~^3P _{0}$&  1.016E+02 &           &          &  1.056E-10 &            &   \\
$1s\,8p ~^3P_{2}$ &  $1s\,4p ~^3P_{1}$&  6.636E+02 &           &          &  3.843E-10 &            &   \\
$1s\,8s ~^3S_{1}$ &  $1s\,4s ~^1S _{0}$&  1.682E+03 &           &          &  1.758E-09 &            &   \\
$1s\,8p ~^1P_{1}$ &  $1s\,4p ~^3P_{2}$&  2.754E+03 &           &          &  5.762E-10 &            &   \\
$1s\,8d ~^1D_{2}$ &  $1s\,4d ~^3D_{1}$&  6.246E+02 &           &          &   3.67E-10 &            &   \\
$1s\,8d ~^3D_{1}$ &  $1s\,4d ~^3D_{2}$&  2.915E+04 &           &          &  6.168E-09 &            &   \\
$1s\,8d ~^3D_{2}$ &  $1s\,4d ~^3D_{1}$&  1.735E+04 &           &          &   1.02E-08 &            &   \\
$1s\,8d ~^1D_{2}$ &  $1s\,4d ~^3D_{3}$&  1.084E+03 &           &          &  2.736E-10 &            &   \\
$1s\,8f ~^3F_{2}$ &  $1s\,4f ~^3F_{3}$&  1.014E+04 &           &          &   2.56E-09 &            &   \\
$1s\,8f ~^3F_{3}$ &  $1s\,4f ~^3F_{2}$&  7.298E+03 &           &          &  3.612E-09 &            &   \\
$1s\,8d ~^3D_{3}$ &  $1s\,4d ~^1D_{2}$&  8.735E+02 &           &          &  4.324E-10 &            &   \\
$1s\,8f ~^1F_{3}$ &  $1s\,4f ~^3F_{4}$&  4.236E+03 &           &          &  1.166E-09 &            &   \\
$1s\,8p ~^3P_{2}$ &  $1s\,4p ~^1P_{1}$&  4.203E+02 &           &          &  2.479E-10 &            &   \\
$1s\,8f ~^3F_{4}$ &  $1s\,4f ~^1F_{3}$&  3.320E+03 &           &          &  1.511E-09 &            &   \\
$1s\,7s ~^1S _{0}$ &  $1s\,4s ~^3S_{1}$&  1.748E+04 &           &          &  2.453E-09 &            &   \\
$1s\,7p ~^3P_{2}$ &  $1s\,4p ~^3P_{1}$&  1.638E+03 &           &          &  1.175E-09 &            &   \\
$1s\,7p ~^1P_{1}$ &  $1s\,4p ~^3P_{2}$&  8.856E+03 &           &          &  2.294E-09 &            &   \\
$1s\,7s ~^3S_{1}$ &  $1s\,4s ~^1S _{0}$&  3.821E+03 &           &          &  4.957E-09 &            &   \\
$1s\,7p ~^3P_{1}$ &  $1s\,4p ~^3P_{2}$&  4.026E+02 &           &          &  1.047E-10 &            &   \\
$1s\,7d ~^1D_{2}$ &  $1s\,4d ~^3D_{1}$&  6.057E+02 &           &          &  4.413E-10 &            &   \\
$1s\,7d ~^3D_{1}$ &  $1s\,4d ~^3D_{2}$&  2.782E+04 &           &          &    7.3E-09 &            &   \\
$1s\,7d ~^3D_{2}$ &  $1s\,4d ~^3D_{1}$&  1.657E+04 &           &          &  1.208E-08 &            &   \\
$1s\,7f ~^3F_{2}$ &  $1s\,4f ~^3F_{3}$&  1.026E+04 &           &          &  3.213E-09 &            &   \\
$1s\,7f ~^3F_{3}$ &  $1s\,4f ~^3F_{2}$&  7.396E+03 &           &          &   4.54E-09 &            &   \\
$1s\,7d ~^3D_{3}$ &  $1s\,4d ~^1D_{2}$&  2.211E+02 &           &          &  1.358E-10 &            &   \\
$1s\,7f ~^1F_{3}$ &  $1s\,4f ~^3F_{4}$&  3.589E+03 &           &          &  1.226E-09 &            &   \\
$1s\,7f ~^3F_{4}$ &  $1s\,4f ~^1F_{3}$&  2.820E+03 &           &          &  1.591E-09 &            &   \\
$1s\,7p ~^3P_{2}$ &  $1s\,4p ~^1P_{1}$&  2.962E+03 &           &          &  2.169E-09 &            &   \\
$1s\,6s ~^1S _{0}$ &  $1s\,4s ~^3S_{1}$&  3.144E+04 &           &          &   6.45E-09 &            &   \\
$1s\,6p ~^3P_{2}$ &  $1s\,4p ~^3P_{1}$&  3.183E+03 &           &          &   3.35E-09 &            &   \\
$1s\,6p ~^3P_{1}$ &  $1s\,4p ~^3P _{0}$&  7.565E+02 &           &          &  1.434E-09 &            &   \\
$1s\,6p ~^1P_{1}$ &  $1s\,4p ~^3P_{2}$&  1.914E+04 &           &          &  7.266E-09 &            &   \\
$1s\,6p ~^3P _{0}$ &  $1s\,4p ~^3P_{1}$&  1.318E+03 &           &          &   2.78E-10 &            &   \\
$1s\,6p ~^3P_{1}$ &  $1s\,4p ~^3P_{2}$&  1.356E+03 &           &          &  5.184E-10 &            &   \\
$1s\,6s ~^3S_{1}$ &  $1s\,4s ~^1S _{0}$&  8.113E+03 &           &          &  1.552E-08 &            &   \\
$1s\,6d ~^1D_{2}$ &  $1s\,4d ~^3D_{1}$&  6.327E+02 &           &          &   6.77E-10 &            &   \\
$1s\,6d ~^3D_{1}$ &  $1s\,4d ~^3D_{2}$&  2.900E+04 &           &          &  1.118E-08 &            &   \\
$1s\,6d ~^3D_{2}$ &  $1s\,4d ~^3D_{1}$&  1.730E+04 &           &          &  1.853E-08 &            &   \\
$1s\,6f ~^3F_{2}$ &  $1s\,4f ~^3F_{3}$&  1.212E+04 &           &          &   5.58E-09 &            &   \\
$1s\,6f ~^3F_{3}$ &  $1s\,4f ~^3F_{2}$&  8.750E+03 &           &          &  7.894E-09 &            &   \\
$1s\,6f ~^1F_{3}$ &  $1s\,4f ~^3F_{4}$&  4.674E+03 &           &          &  2.344E-09 &            &   \\
$1s\,6d ~^3D_{1}$ &  $1s\,4d ~^1D_{2}$&  2.832E+02 &           &          &  1.096E-10 &            &   \\
$1s\,6f ~^3F_{4}$ &  $1s\,4f ~^1F_{3}$&  3.674E+03 &           &          &  3.047E-09 &            &   \\
$1s\,6p ~^3P_{2}$ &  $1s\,4p ~^1P_{1}$&  8.123E+03 &           &          &  8.763E-09 &            &   \\
$1s\,6p ~^3P _{0}$ &  $1s\,4p ~^1P_{1}$&  1.339E+03 &           &          &  2.897E-10 &            &   \\
$1s\,8s ~^1S _{0}$ &  $1s\,5s ~^3S_{1}$&  5.706E+03 &           &          &  2.403E-09 &            &   \\
$1s\,8p ~^1P_{1}$ &  $1s\,5p ~^3P _{0}$&  2.101E+02 &           &          &  8.079E-10 &            &   \\
$1s\,8p ~^3P_{1}$ &  $1s\,5p ~^3P _{0}$&  4.419E+02 &           &          &  1.707E-09 &            &   \\
$1s\,8p ~^3P _{0}$ &  $1s\,5p ~^3P_{1}$&  1.690E+03 &           &          &   7.26E-10 &            &   \\
$1s\,8s ~^3S_{1}$ &  $1s\,5s ~^1S _{0}$&  1.347E+03 &           &          &  5.229E-09 &            &   \\
$1s\,8d ~^1D_{2}$ &  $1s\,5d ~^3D_{1}$&  1.096E+02 &           &          &  2.381E-10 &            &   \\
$1s\,8d ~^3D_{2}$ &  $1s\,5d ~^3D_{1}$&  2.749E+03 &           &          &  5.977E-09 &            &   \\
$1s\,8d ~^3D_{1}$ &  $1s\,5d ~^3D_{2}$&  4.609E+03 &           &          &  3.608E-09 &            &   \\
$1s\,8d ~^1D_{2}$ &  $1s\,5d ~^3D_{3}$&  1.381E+03 &           &          &  1.289E-09 &            &   \\
$1s\,8f ~^3F_{2}$ &  $1s\,5f ~^3F_{3}$&  2.138E+03 &           &          &  1.996E-09 &            &   \\
$1s\,8f ~^3F_{3}$ &  $1s\,5f ~^3F_{2}$&  1.544E+03 &           &          &  2.826E-09 &            &   \\
$1s\,8d ~^3D_{3}$ &  $1s\,5d ~^1D_{2}$&  1.045E+03 &           &          &  1.914E-09 &            &   \\
$1s\,8f ~^1F_{3}$ &  $1s\,5f ~^3F_{4}$&  2.022E+02 &           &          &  2.058E-10 &            &   \\
$1s\,8g ~^3G_{3}$ &  $1s\,5g ~^3G_{4}$&  2.593E+03 &           &          &  2.639E-09 &            &   \\
$1s\,8g ~^3G_{4}$ &  $1s\,5g ~^3G_{3}$&  2.024E+03 &           &          &  3.406E-09 &            &   \\
$1s\,8f ~^3F_{4}$ &  $1s\,5f ~^1F_{3}$&  1.610E+02 &           &          &  2.709E-10 &            &   \\
$1s\,8g ~^1G_{4}$ &  $1s\,5g ~^3G_{5}$&  5.351E+02 &           &          &  5.731E-10 &            &   \\
$1s\,8g ~^3G_{5}$ &  $1s\,5g ~^1G_{4}$&  4.403E+02 &           &          &  7.046E-10 &            &   \\
$1s\,8p ~^3P_{2}$ &  $1s\,5p ~^1P_{1}$&  6.158E+01 &           &          &  1.345E-10 &            &   \\
$1s\,5s ~^1S _{0}$ &  $1s\,4s ~^3S_{1}$&  5.138E+04 &           &          &  2.471E-08 &            &   \\
$1s\,5p ~^1P_{1}$ &  $1s\,4p ~^3P_{2}$&  2.659E+04 &           &          &  2.382E-08 &            &   \\
$1s\,5p ~^3P_{2}$ &  $1s\,4p ~^3P_{1}$&  4.370E+03 &           &          &   1.09E-08 &            &   \\
$1s\,5p ~^3P_{1}$ &  $1s\,4p ~^3P _{0}$&  5.791E+02 &           &          &  2.608E-09 &            &   \\
$1s\,5p ~^3P _{0}$ &  $1s\,4p ~^3P_{1}$&  9.081E+02 &           &          &   4.56E-10 &            &   \\
$1s\,5p ~^3P_{1}$ &  $1s\,4p ~^3P_{2}$&  2.247E+03 &           &          &  2.052E-09 &            &   \\
$1s\,5d ~^1D_{2}$ &  $1s\,4d ~^3D_{1}$&  7.419E+02 &           &          &  1.886E-09 &            &   \\
$1s\,5d ~^3D_{1}$ &  $1s\,4d ~^3D_{2}$&  3.637E+04 &           &          &   3.34E-08 &            &   \\
$1s\,5d ~^3D_{2}$ &  $1s\,4d ~^3D_{1}$&  2.174E+04 &           &          &  5.547E-08 &            &   \\
$1s\,5f ~^3F_{2}$ &  $1s\,4f ~^3F_{3}$&  1.942E+04 &           &          &  2.129E-08 &            &   \\
$1s\,5f ~^3F_{3}$ &  $1s\,4f ~^3F_{2}$&  1.401E+04 &           &          &   3.01E-08 &            &   \\
$1s\,5f ~^1F_{3}$ &  $1s\,4f ~^3F_{4}$&  6.272E+03 &           &          &  7.493E-09 &            &   \\
$1s\,5s ~^3S_{1}$ &  $1s\,4s ~^1S _{0}$&  1.567E+04 &           &          &  7.224E-08 &            &   \\
$1s\,5f ~^3F_{4}$ &  $1s\,4f ~^1F_{3}$&  4.929E+03 &           &          &   9.74E-09 &            &   \\
$1s\,5d ~^3D_{1}$ &  $1s\,4d ~^1D_{2}$&  3.769E+02 &           &          &  3.482E-10 &            &   \\
$1s\,5p ~^3P_{2}$ &  $1s\,4p ~^1P_{1}$&  1.194E+04 &           &          &  3.095E-08 &            &   \\
$1s\,5p ~^3P _{0}$ &  $1s\,4p ~^1P_{1}$&  1.438E+03 &           &          &   7.51E-10 &            &   \\
$1s\,7s ~^1S _{0}$ &  $1s\,5s ~^3S_{1}$&  9.805E+03 &           &          &  6.357E-09 &            &   \\
$1s\,7p ~^1P_{1}$ &  $1s\,5p ~^3P _{0}$&  1.768E+02 &           &          &  1.047E-09 &            &   \\
$1s\,7p ~^3P_{2}$ &  $1s\,5p ~^3P_{1}$&  9.712E+01 &           &          &  3.219E-10 &            &   \\
$1s\,7p ~^1P_{1}$ &  $1s\,5p ~^3P_{2}$&  2.541E+02 &           &          &  3.034E-10 &            &   \\
$1s\,7p ~^3P_{1}$ &  $1s\,5p ~^3P _{0}$&  3.142E+02 &           &          &  1.877E-09 &            &   \\
$1s\,7p ~^3P _{0}$ &  $1s\,5p ~^3P_{1}$&  1.277E+03 &           &          &  8.493E-10 &            &   \\
$1s\,7s ~^3S_{1}$ &  $1s\,5s ~^1S _{0}$&  2.629E+03 &           &          &  1.585E-08 &            &   \\
$1s\,7d ~^1D_{2}$ &  $1s\,5d ~^3D_{1}$&  7.890E+01 &           &          &  2.651E-10 &            &   \\
$1s\,7d ~^3D_{2}$ &  $1s\,5d ~^3D_{1}$&  1.813E+03 &           &          &    6.1E-09 &            &   \\
$1s\,7d ~^3D_{1}$ &  $1s\,5d ~^3D_{2}$&  3.038E+03 &           &          &   3.68E-09 &            &   \\
$1s\,7d ~^1D_{2}$ &  $1s\,5d ~^3D_{3}$&  4.030E+02 &           &          &  5.819E-10 &            &   \\
$1s\,7f ~^3F_{2}$ &  $1s\,5f ~^3F_{3}$&  1.473E+03 &           &          &  2.129E-09 &            &   \\
$1s\,7f ~^3F_{3}$ &  $1s\,5f ~^3F_{2}$&  1.069E+03 &           &          &  3.028E-09 &            &   \\
$1s\,7d ~^3D_{3}$ &  $1s\,5d ~^1D_{2}$&  3.230E+02 &           &          &  9.154E-10 &            &   \\
$1s\,7f ~^1F_{3}$ &  $1s\,5f ~^3F_{4}$&  4.022E+02 &           &          &  6.336E-10 &            &   \\
$1s\,7g ~^3G_{3}$ &  $1s\,5g ~^3G_{4}$&  3.015E+03 &           &          &   4.75E-09 &            &   \\
$1s\,7g ~^3G_{4}$ &  $1s\,5g ~^3G_{3}$&  2.356E+03 &           &          &  6.134E-09 &            &   \\
$1s\,7f ~^3F_{4}$ &  $1s\,5f ~^1F_{3}$&  3.188E+02 &           &          &  8.304E-10 &            &   \\
$1s\,7g ~^1G_{4}$ &  $1s\,5g ~^3G_{5}$&  5.324E+02 &           &          &  8.827E-10 &            &   \\
$1s\,7g ~^3G_{5}$ &  $1s\,5g ~^1G_{4}$&  4.387E+02 &           &          &  1.087E-09 &            &   \\
$1s\,7p ~^3P_{2}$ &  $1s\,5p ~^1P_{1}$&  3.021E+01 &           &          &  1.024E-10 &            &   \\
$1s\,6s ~^1S _{0}$ &  $1s\,5s ~^3S_{1}$&  1.371E+04 &           &          &  2.249E-08 &            &   \\
$1s\,6p ~^1P_{1}$ &  $1s\,5p ~^3P _{0}$&  6.915E+01 &           &          &  1.038E-09 &            &   \\
$1s\,6p ~^1P_{1}$ &  $1s\,5p ~^3P_{2}$&  1.201E+02 &           &          &  3.652E-10 &            &   \\
$1s\,8s ~^1S _{0}$ &  $1s\,6s ~^3S_{1}$&  2.464E+03 &           &          &   4.17E-09 &            &   \\
$1s\,6p ~^3P_{2}$ &  $1s\,5p ~^3P_{1}$&  6.489E+01 &           &          &    5.5E-10 &            &   \\
$1s\,6p ~^3P_{1}$ &  $1s\,5p ~^3P _{0}$&  4.092E+01 &           &          &   6.27E-10 &            &   \\
$1s\,6p ~^3P _{0}$ &  $1s\,5p ~^3P_{1}$&  2.482E+02 &           &          &   4.24E-10 &            &   \\
$1s\,8p ~^1P_{1}$ &  $1s\,6p ~^3P _{0}$&  3.085E+02 &           &          &  4.759E-09 &            &   \\
$1s\,6d ~^1D_{2}$ &  $1s\,5d ~^3D_{1}$&  5.150E+01 &           &          &  4.437E-10 &            &   \\
$1s\,8p ~^1P_{1}$ &  $1s\,6p ~^3P_{2}$&  2.828E+02 &           &          &  8.788E-10 &            &   \\
$1s\,8p ~^3P_{1}$ &  $1s\,6p ~^3P _{0}$&  2.079E+03 &           &          &  3.236E-08 &            &   \\
$1s\,6d ~^3D_{2}$ &  $1s\,5d ~^3D_{1}$&  1.062E+03 &           &          &  9.187E-09 &            &   \\
$1s\,6d ~^3D_{1}$ &  $1s\,5d ~^3D_{2}$&  1.779E+03 &           &          &  5.538E-09 &            &   \\
$1s\,6d ~^1D_{2}$ &  $1s\,5d ~^3D_{3}$&  1.903E+02 &           &          &  7.056E-10 &            &   \\
$1s\,8p ~^3P _{0}$ &  $1s\,6p ~^3P_{1}$&  5.818E+03 &           &          &  1.008E-08 &            &   \\
$1s\,6f ~^3F_{2}$ &  $1s\,5f ~^3F_{3}$&  9.731E+02 &           &          &  3.613E-09 &            &   \\
$1s\,6f ~^3F_{3}$ &  $1s\,5f ~^3F_{2}$&  7.088E+02 &           &          &   5.16E-09 &            &   \\
$1s\,6f ~^1F_{3}$ &  $1s\,5f ~^3F_{4}$&  7.760E+01 &           &          &  3.141E-10 &            &   \\
$1s\,6g ~^3G_{3}$ &  $1s\,5g ~^3G_{4}$&  5.009E+03 &           &          &  2.028E-08 &            &   \\
$1s\,6d ~^3D_{3}$ &  $1s\,5d ~^1D_{2}$&  1.605E+02 &           &          &   1.17E-09 &            &   \\
$1s\,6g ~^3G_{4}$ &  $1s\,5g ~^3G_{3}$&  3.911E+03 &           &          &  2.617E-08 &            &   \\
$1s\,6f ~^3F_{4}$ &  $1s\,5f ~^1F_{3}$&  6.314E+01 &           &          &  4.226E-10 &            &   \\
$1s\,6g ~^1G_{4}$ &  $1s\,5g ~^3G_{5}$&  6.621E+02 &           &          &  2.821E-09 &            &   \\
$1s\,6g ~^3G_{5}$ &  $1s\,5g ~^1G_{4}$&  5.456E+02 &           &          &  3.473E-09 &            &   \\
$1s\,8p ~^3P_{1}$ &  $1s\,6p ~^3P_{2}$&  1.332E+02 &           &          &  4.176E-10 &            &   \\
$1s\,6s ~^3S_{1}$ &  $1s\,5s ~^1S _{0}$&  4.196E+03 &           &          &  6.586E-08 &            &   \\
$1s\,8s ~^3S_{1}$ &  $1s\,6s ~^1S _{0}$&  6.640E+02 &           &          &  1.044E-08 &            &   \\
$1s\,8d ~^3D_{2}$ &  $1s\,6d ~^3D_{1}$&  1.163E+02 &           &          &  1.018E-09 &            &   \\
$1s\,8d ~^3D_{1}$ &  $1s\,6d ~^3D_{2}$&  1.956E+02 &           &          &   6.16E-10 &            &   \\
$1s\,8f ~^3F_{2}$ &  $1s\,6f ~^3F_{3}$&  4.178E+01 &           &          &   1.57E-10 &            &   \\
$1s\,8f ~^3F_{3}$ &  $1s\,6f ~^3F_{2}$&  3.133E+01 &           &          &  2.308E-10 &            &   \\
$1s\,8d ~^3D_{3}$ &  $1s\,6d ~^1D_{2}$&  2.310E+01 &           &          &  1.702E-10 &            &   \\
$1s\,8g ~^3G_{3}$ &  $1s\,6g ~^3G_{4}$&  5.968E+02 &           &          &  2.443E-09 &            &   \\
$1s\,8g ~^3G_{4}$ &  $1s\,6g ~^3G_{3}$&  4.671E+02 &           &          &  3.161E-09 &            &   \\
$1s\,8g ~^1G_{4}$ &  $1s\,6g ~^3G_{5}$&  6.156E+01 &           &          &  2.653E-10 &            &   \\
$1s\,8h ~^3H_{4}$ &  $1s\,6h ~^3H_{5}$&  1.253E+03 &           &          &  5.399E-09 &            &   \\
$1s\,8h ~^3H_{5}$ &  $1s\,6h ~^3H_{4}$&  1.027E+03 &           &          &  6.611E-09 &            &   \\
$1s\,8g ~^3G_{5}$ &  $1s\,6g ~^1G_{4}$&  5.101E+01 &           &          &  3.283E-10 &            &   \\
$1s\,8h ~^1H_{5}$ &  $1s\,6h ~^3H_{6}$&  2.407E+02 &           &          &  1.073E-09 &            &   \\
$1s\,8h ~^3H_{6}$ &  $1s\,6h ~^1H_{5}$&  2.043E+02 &           &          &  1.272E-09 &            &   \\
$1s\,8p ~^3P_{2}$ &  $1s\,6p ~^1P_{1}$&  2.908E+02 &           &          &  2.564E-09 &            &   \\
$1s\,8p ~^3P _{0}$ &  $1s\,6p ~^1P_{1}$&  1.268E+03 &           &          &  2.243E-09 &            &   \\
$1s\,7s ~^1S _{0}$ &  $1s\,6s ~^3S_{1}$&  3.480E+03 &           &          &  1.577E-08 &            &   \\
$1s\,7p ~^1P_{1}$ &  $1s\,6p ~^3P _{0}$&  3.815E+02 &           &          &  1.578E-08 &            &   \\
$1s\,7p ~^1P_{1}$ &  $1s\,6p ~^3P_{2}$&  4.150E+01 &           &          &  3.474E-10 &            &   \\
$1s\,7p ~^3P_{1}$ &  $1s\,6p ~^3P _{0}$&  2.610E+03 &           &          &  1.103E-07 &            &   \\
$1s\,7p ~^3P _{0}$ &  $1s\,6p ~^3P_{1}$&  7.412E+03 &           &          &   3.49E-08 &            &   \\
$1s\,7p ~^3P_{1}$ &  $1s\,6p ~^3P_{2}$&  4.900E+01 &           &          &  4.192E-10 &            &   \\
$1s\,7d ~^1D_{2}$ &  $1s\,6d ~^3D_{3}$&  5.350E+01 &           &          &  5.456E-10 &            &   \\
$1s\,7f ~^3F_{2}$ &  $1s\,6f ~^3F_{3}$&  1.918E+01 &           &          &  1.959E-10 &            &   \\
$1s\,7f ~^3F_{3}$ &  $1s\,6f ~^3F_{2}$&  1.276E+01 &           &          &  2.554E-10 &            &   \\
$1s\,7g ~^3G_{3}$ &  $1s\,6g ~^3G_{4}$&  4.341E+02 &           &          &  4.832E-09 &            &   \\
$1s\,7g ~^3G_{4}$ &  $1s\,6g ~^3G_{3}$&  3.402E+02 &           &          &  6.261E-09 &            &   \\
$1s\,7d ~^3D_{3}$ &  $1s\,6d ~^1D_{2}$&  4.436E+01 &           &          &   8.89E-10 &            &   \\
$1s\,7g ~^1G_{4}$ &  $1s\,6g ~^3G_{5}$&  1.129E+01 &           &          &  1.323E-10 &            &   \\
$1s\,7h ~^3H_{4}$ &  $1s\,6h ~^3H_{5}$&  1.951E+03 &           &          &  2.286E-08 &            &   \\
$1s\,7h ~^3H_{5}$ &  $1s\,6h ~^3H_{4}$&  1.599E+03 &           &          &  2.799E-08 &            &   \\
$1s\,7g ~^3G_{5}$ &  $1s\,6g ~^1G_{4}$&  9.523E+00 &           &          &  1.667E-10 &            &   \\
$1s\,7h ~^1H_{5}$ &  $1s\,6h ~^3H_{6}$&  1.715E+02 &           &          &  2.078E-09 &            &   \\
$1s\,7h ~^3H_{6}$ &  $1s\,6h ~^1H_{5}$&  1.457E+02 &           &          &  2.467E-09 &            &   \\
$1s\,7s ~^3S_{1}$ &  $1s\,6s ~^1S _{0}$&  1.065E+03 &           &          &  4.616E-08 &            &   \\
$1s\,7p ~^3P_{2}$ &  $1s\,6p ~^1P_{1}$&  6.001E+01 &           &          &  1.452E-09 &            &   \\
$1s\,7p ~^3P _{0}$ &  $1s\,6p ~^1P_{1}$&  1.628E+03 &           &          &   7.94E-09 &            &   \\
$1s\,8s ~^1S _{0}$ &  $1s\,7s ~^3S_{1}$&  9.248E+02 &           &          &  9.977E-09 &            &   \\
$1s\,8p ~^1P_{1}$ &  $1s\,7p ~^3P _{0}$&  1.011E+02 &           &          &  9.939E-09 &            &   \\
$1s\,8p ~^1P_{1}$ &  $1s\,7p ~^3P_{2}$&  1.776E+03 &           &          &  3.532E-08 &            &   \\
$1s\,8p ~^3P_{2}$ &  $1s\,7p ~^3P_{1}$&  2.305E+02 &           &          &  1.281E-08 &            &   \\
$1s\,8p ~^3P_{1}$ &  $1s\,7p ~^3P _{0}$&  6.746E+02 &           &          &  6.779E-08 &            &   \\
$1s\,8p ~^3P _{0}$ &  $1s\,7p ~^3P_{1}$&  1.914E+03 &           &          &  2.144E-08 &            &   \\
$1s\,8d ~^3D_{2}$ &  $1s\,7d ~^3D_{1}$&  3.399E+01 &           &          &   1.92E-09 &            &   \\
$1s\,8d ~^3D_{1}$ &  $1s\,7d ~^3D_{2}$&  5.631E+01 &           &          &  1.145E-09 &            &   \\
$1s\,8d ~^1D_{2}$ &  $1s\,7d ~^3D_{3}$&  8.672E+01 &           &          &    2.1E-09 &            &   \\
$1s\,8p ~^3P_{1}$ &  $1s\,7p ~^3P_{2}$&  2.481E+02 &           &          &  5.046E-09 &            &   \\
$1s\,8f ~^3F_{2}$ &  $1s\,7f ~^3F_{3}$&  7.683E+01 &           &          &  1.863E-09 &            &   \\
$1s\,8f ~^3F_{3}$ &  $1s\,7f ~^3F_{2}$&  5.384E+01 &           &          &   2.56E-09 &            &   \\
$1s\,8f ~^1F_{3}$ &  $1s\,7f ~^3F_{4}$&  5.212E+01 &           &          &  1.377E-09 &            &   \\
$1s\,8g ~^3G_{4}$ &  $1s\,7g ~^3G_{3}$&  2.657E+00 &           &          &  1.161E-10 &            &   \\
$1s\,8f ~^3F_{4}$ &  $1s\,7f ~^1F_{3}$&  4.112E+01 &           &          &  1.797E-09 &            &   \\
$1s\,8g ~^1G_{4}$ &  $1s\,7g ~^3G_{5}$&  2.393E+01 &           &          &  6.655E-10 &            &   \\
$1s\,8h ~^3H_{4}$ &  $1s\,7h ~^3H_{5}$&  1.706E+02 &           &          &  4.744E-09 &            &   \\
$1s\,8d ~^3D_{3}$ &  $1s\,7d ~^1D_{2}$&  6.584E+01 &           &          &  3.134E-09 &            &   \\
$1s\,8h ~^3H_{5}$ &  $1s\,7h ~^3H_{4}$&  1.401E+02 &           &          &  5.821E-09 &            &   \\
$1s\,8g ~^3G_{5}$ &  $1s\,7g ~^1G_{4}$&  1.980E+01 &           &          &  8.229E-10 &            &   \\
$1s\,8h ~^1H_{5}$ &  $1s\,7h ~^3H_{6}$&  1.302E+02 &           &          &  3.745E-09 &            &   \\
$1s\,8i ~^3I_{5}$ &  $1s\,7i ~^3I_{6}$&  3.387E+01 &           &          &  9.746E-10 &            &   \\
$1s\,8i ~^3I_{6}$ &  $1s\,7i ~^3I_{5}$&  2.879E+01 &           &          &  1.157E-09 &            &   \\
$1s\,8h ~^3H_{6}$ &  $1s\,7h ~^1H_{5}$&  1.098E+02 &           &          &  4.411E-09 &            &   \\
$1s\,8i ~^1I_{6}$ &  $1s\,7i ~^3I_{7}$&  1.321E+02 &           &          &  3.893E-09 &            &   \\
$1s\,8i ~^3I_{7}$ &  $1s\,7i ~^1I_{6}$&  1.147E+02 &           &          &    4.5E-09 &            &   \\
$1s\,8d ~^3D_{2}$ &  $1s\,7d ~^3D_{3}$&  5.095E+00 &           &          &  1.238E-10 &            &   \\
$1s\,8s ~^3S_{1}$ &  $1s\,7s ~^1S _{0}$&  2.838E+02 &           &          &  2.927E-08 &            &   \\
$1s\,8p ~^3P_{2}$ &  $1s\,7p ~^1P_{1}$&  9.187E+02 &           &          &   5.28E-08 &            &   \\
$1s\,8p ~^3P _{0}$ &  $1s\,7p ~^1P_{1}$&  4.311E+02 &           &          &  4.997E-09 &            &   \\
$1s\,2s ~^1S _{0}$ &  $1s\,2s ~^3S_{1}$&  2.689E+01 &        2.296E+01 &          &  3.463E-10 &  2.964E-10 &   \\
$1s\,2p ~^1P_{1}$ &  $1s\,2p ~^3P _{0}$&  3.585E+03 &           &          &  5.162E-07 &            &   \\
$1s\,2p ~^1P_{1}$ &  $1s\,2p ~^3P_{2}$&  1.304E+03 &           &          &  7.762E-08 &            &   \\
$1s\,3s ~^1S _{0}$ &  $1s\,3s ~^3S_{1}$&  9.071E-01 &           &          &  1.674E-10 &            &   \\
$1s\,3p ~^1P_{1}$ &  $1s\,3p ~^3P _{0}$&  8.938E+01 &           &          &  1.657E-07 &            &   \\
$1s\,2p ~^3P_{2}$ &  $1s\,2p ~^3P_{1}$&  1.155E+03 &           &          &  1.439E-06 &            &   \\
$1s\,3p ~^1P_{1}$ &  $1s\,3p ~^3P_{2}$&  2.944E+01 &           &          &    2.4E-08 &            &   \\
$1s\,4p ~^1P_{1}$ &  $1s\,4p ~^3P _{0}$&  6.476E+00 &           &          &  7.031E-08 &            &   \\
$1s\,4p ~^1P_{1}$ &  $1s\,4p ~^3P_{2}$&  2.008E+00 &           &          &   9.79E-09 &            &   \\
$1s\,3p ~^3P_{2}$ &  $1s\,3p ~^3P_{1}$&  3.052E+01 &           &          &  4.277E-07 &            &   \\
$1s\,5p ~^1P_{1}$ &  $1s\,5p ~^3P _{0}$&  8.619E-01 &           &          &  3.635E-08 &            &   \\
$1s\,2p ~^3P_{1}$ &  $1s\,2p ~^3P _{0}$&  1.268E+01 &           &          &  6.958E-07 &            &   \\
$1s\,5p ~^1P_{1}$ &  $1s\,5p ~^3P_{2}$&  2.813E-01 &           &          &  5.378E-09 &            &   \\
$1s\,3d ~^1D_{2}$ &  $1s\,3d ~^3D_{1}$&  2.155E+00 &           &          &  1.198E-07 &            &   \\
$1s\,6p ~^1P_{1}$ &  $1s\,6p ~^3P _{0}$&  1.707E-01 &           &          &  2.169E-08 &            &   \\
$1s\,4p ~^3P_{2}$ &  $1s\,4p ~^3P_{1}$&  2.291E+00 &           &          &  1.798E-07 &            &   \\
$1s\,3d ~^3D_{3}$ &  $1s\,3d ~^3D_{2}$&  1.881E+00 &           &          &  1.406E-07 &            &   \\
$1s\,6p ~^1P_{1}$ &  $1s\,6p ~^3P_{2}$&  5.380E-02 &           &          &   3.11E-09 &            &   \\
$1s\,7p ~^1P_{1}$ &  $1s\,7p ~^3P _{0}$&  4.135E-02 &           &          &  1.328E-08 &            &   \\
$1s\,4d ~^1D_{2}$ &  $1s\,4d ~^3D_{1}$&  1.706E-01 &           &          &  4.833E-08 &            &   \\
$1s\,5p ~^3P_{2}$ &  $1s\,5p ~^3P_{1}$&  3.089E-01 &           &          &  9.243E-08 &            &   \\
$1s\,3p ~^3P_{1}$ &  $1s\,3p ~^3P _{0}$&  3.260E-01 &           &          &  2.041E-07 &            &   \\
$1s\,8p ~^1P_{1}$ &  $1s\,8p ~^3P _{0}$&  1.212E-02 &           &          &  8.645E-09 &            &   \\
$1s\,7p ~^1P_{1}$ &  $1s\,7p ~^3P_{2}$&  1.221E-02 &           &          &  1.786E-09 &            &   \\
$1s\,4d ~^3D_{3}$ &  $1s\,4d ~^3D_{2}$&  1.355E-01 &           &          &  5.992E-08 &            &   \\
$1s\,6p ~^3P_{2}$ &  $1s\,6p ~^3P_{1}$&  5.974E-02 &           &          &  5.343E-08 &            &   \\
$1s\,8p ~^1P_{1}$ &  $1s\,8p ~^3P_{2}$&  4.293E-03 &           &          &  1.391E-09 &            &   \\
$1s\,3d ~^1D_{2}$ &  $1s\,3d ~^3D_{3}$&  2.726E-02 &           &          &    1.2E-08 &            &   \\
$1s\,5d ~^1D_{2}$ &  $1s\,5d ~^3D_{1}$&  2.346E-02 &           &          &  2.433E-08 &            &   \\
$1s\,4f ~^3F_{4}$ &  $1s\,4f ~^3F_{3}$&  2.144E-02 &           &          &   2.73E-08 &            &   \\
$1s\,4f ~^1F_{3}$ &  $1s\,4f ~^3F_{2}$&  1.935E-02 &           &          &  2.796E-08 &            &   \\
$1s\,4p ~^3P_{1}$ &  $1s\,4p ~^3P _{0}$&  2.448E-02 &           &          &  8.635E-08 &            &   \\
$1s\,5d ~^3D_{3}$ &  $1s\,5d ~^3D_{2}$&  1.790E-02 &           &          &  3.082E-08 &            &   \\
$1s\,7p ~^3P_{2}$ &  $1s\,7p ~^3P_{1}$&  1.479E-02 &           &          &  3.343E-08 &            &   \\
$1s\,6d ~^1D_{2}$ &  $1s\,6d ~^3D_{1}$&  4.604E-03 &           &          &  1.397E-08 &            &   \\
$1s\,4d ~^1D_{2}$ &  $1s\,4d ~^3D_{3}$&  3.242E-03 &           &          &   5.43E-09 &            &   \\
$1s\,8p ~^3P_{2}$ &  $1s\,8p ~^3P_{1}$&  4.470E-03 &           &          &   2.26E-08 &            &   \\
$1s\,6d ~^3D_{3}$ &  $1s\,6d ~^3D_{2}$&  3.433E-03 &           &          &  1.785E-08 &            &   \\
$1s\,5f ~^3F_{4}$ &  $1s\,5f ~^3F_{3}$&  2.869E-03 &           &          &  1.401E-08 &            &   \\
$1s\,5f ~^1F_{3}$ &  $1s\,5f ~^3F_{2}$&  2.607E-03 &           &          &  1.428E-08 &            &   \\
$1s\,5p ~^3P_{1}$ &  $1s\,5p ~^3P _{0}$&  3.277E-03 &           &          &  4.414E-08 &            &   \\
$1s\,7d ~^1D_{2}$ &  $1s\,7d ~^3D_{1}$&  1.158E-03 &           &          &   8.75E-09 &            &   \\
$1s\,5d ~^1D_{2}$ &  $1s\,5d ~^3D_{3}$&  5.270E-04 &           &          &  2.901E-09 &            &   \\
$1s\,7d ~^3D_{3}$ &  $1s\,7d ~^3D_{2}$&  8.517E-04 &           &          &  1.124E-08 &            &   \\
$1s\,8d ~^1D_{2}$ &  $1s\,8d ~^3D_{1}$&  3.493E-04 &           &          &  5.847E-09 &            &   \\
$1s\,5g ~^3G_{5}$ &  $1s\,5g ~^3G_{4}$&  6.438E-04 &           &          &  8.238E-09 &            &   \\
$1s\,5g ~^1G_{4}$ &  $1s\,5g ~^3G_{3}$&  5.960E-04 &           &          &  8.397E-09 &            &   \\
$1s\,6f ~^3F_{4}$ &  $1s\,6f ~^3F_{3}$&  5.548E-04 &           &          &  8.116E-09 &            &   \\
$1s\,6f ~^1F_{3}$ &  $1s\,6f ~^3F_{2}$&  5.064E-04 &           &          &   8.25E-09 &            &   \\
$1s\,6p ~^3P_{1}$ &  $1s\,6p ~^3P _{0}$&  6.288E-04 &           &          &  2.527E-08 &            &   \\
$1s\,8d ~^3D_{3}$ &  $1s\,8d ~^3D_{2}$&  2.525E-04 &           &          &  7.482E-09 &            &   \\
$1s\,6d ~^1D_{2}$ &  $1s\,6d ~^3D_{3}$&  1.105E-04 &           &          &  1.687E-09 &            &   \\
$1s\,7f ~^3F_{4}$ &  $1s\,7f ~^3F_{3}$&  1.383E-04 &           &          &  5.114E-09 &            &   \\
$1s\,7f ~^1F_{3}$ &  $1s\,7f ~^3F_{2}$&  1.266E-04 &           &          &   5.19E-09 &            &   \\
$1s\,6g ~^3G_{5}$ &  $1s\,6g ~^3G_{4}$&  1.247E-04 &           &          &  4.768E-09 &            &   \\
$1s\,6g ~^1G_{4}$ &  $1s\,6g ~^3G_{3}$&  1.155E-04 &           &          &  4.859E-09 &            &   \\
$1s\,7p ~^3P_{1}$ &  $1s\,7p ~^3P _{0}$&  1.598E-04 &           &          &  1.614E-08 &            &   \\
$1s\,7d ~^1D_{2}$ &  $1s\,7d ~^3D_{3}$&  2.888E-05 &           &          &  1.065E-09 &            &   \\
$1s\,8f ~^3F_{4}$ &  $1s\,8f ~^3F_{3}$&  4.137E-05 &           &          &  3.423E-09 &            &   \\
$1s\,3d ~^3D_{1}$ &  $1s\,3d ~^3D_{2}$&  1.002E-04 &           &          &  3.872E-09 &            &   \\
$1s\,8f ~^1F_{3}$ &  $1s\,8f ~^3F_{2}$&  3.793E-05 &           &          &   3.47E-09 &            &   \\
$1s\,6h ~^3H_{6}$ &  $1s\,6h ~^3H_{5}$&  3.766E-05 &           &          &  3.142E-09 &            &   \\
$1s\,6h ~^1H_{5}$ &  $1s\,6h ~^3H_{4}$&  3.555E-05 &           &          &  3.182E-09 &            &   \\
$1s\,8p ~^3P_{1}$ &  $1s\,8p ~^3P _{0}$&  4.904E-05 &           &          &  1.096E-08 &            &   \\
$1s\,7g ~^3G_{5}$ &  $1s\,7g ~^3G_{4}$&  3.114E-05 &           &          &  3.002E-09 &            &   \\
$1s\,4f ~^3F_{2}$ &  $1s\,4f ~^3F_{3}$&  5.211E-05 &           &          &  2.963E-09 &            &   \\
$1s\,7g ~^1G_{4}$ &  $1s\,7g ~^3G_{3}$&  2.883E-05 &           &          &  3.059E-09 &            &   \\
$1s\,8d ~^1D_{2}$ &  $1s\,8d ~^3D_{3}$&  8.391E-06 &           &          &  6.707E-10 &            &   \\
$1s\,4f ~^1F_{3}$ &  $1s\,4f ~^3F_{4}$&  1.541E-05 &           &          &  1.426E-09 &            &   \\
$1s\,8g ~^3G_{5}$ &  $1s\,8g ~^3G_{4}$&  9.322E-06 &           &          &  2.009E-09 &            &   \\
$1s\,7h ~^3H_{6}$ &  $1s\,7h ~^3H_{5}$&  9.400E-06 &           &          &  1.978E-09 &            &   \\
$1s\,8g ~^1G_{4}$ &  $1s\,8g ~^3G_{3}$&  8.629E-06 &           &          &  2.046E-09 &            &   \\
$1s\,7h ~^1H_{5}$ &  $1s\,7h ~^3H_{4}$&  8.871E-06 &           &          &  2.003E-09 &            &   \\
$1s\,5f ~^3F_{2}$ &  $1s\,5f ~^3F_{3}$&  6.501E-06 &           &          &  1.473E-09 &            &   \\
$1s\,7i ~^3I_{7}$ &  $1s\,7i ~^3I_{6}$&  3.469E-06 &           &          &  1.401E-09 &            &   \\
$1s\,7i ~^1I_{6}$ &  $1s\,7i ~^3I_{5}$&  3.313E-06 &           &          &  1.414E-09 &            &   \\
$1s\,8h ~^3H_{6}$ &  $1s\,8h ~^3H_{5}$&  2.814E-06 &           &          &  1.324E-09 &            &   \\
$1s\,8h ~^1H_{5}$ &  $1s\,8h ~^3H_{4}$&  2.656E-06 &           &          &   1.34E-09 &            &   \\
$1s\,5f ~^1F_{3}$ &  $1s\,5f ~^3F_{4}$&  2.266E-06 &           &          &  7.441E-10 &            &   \\
$1s\,8i ~^3I_{7}$ &  $1s\,8i ~^3I_{6}$&  1.038E-06 &           &          &  9.369E-10 &            &   \\
$1s\,8i ~^1I_{6}$ &  $1s\,8i ~^3I_{5}$&  9.917E-07 &           &          &  9.455E-10 &            &   \\
$1s\,5g ~^3G_{3}$ &  $1s\,5g ~^3G_{4}$&  1.346E-06 &           &          &  8.926E-10 &            &   \\
$1s\,6f ~^3F_{2}$ &  $1s\,6f ~^3F_{3}$&  1.206E-06 &           &          &  8.383E-10 &            &   \\
$1s\,6f ~^1F_{3}$ &  $1s\,6f ~^3F_{4}$&  4.656E-07 &           &          &   4.38E-10 &            &   \\
$1s\,5g ~^1G_{4}$ &  $1s\,5g ~^3G_{5}$&  4.275E-07 &           &          &  4.705E-10 &            &   \\
$1s\,8k ~^3K_{8}$ &  $1s\,8k ~^3K_{7}$&  4.420E-07 &           &          &   6.98E-10 &            &   \\
$1s\,8k ~^1K_{7}$ &  $1s\,8k ~^3K_{6}$&  4.255E-07 &           &          &  7.025E-10 &            &   \\
$1s\,7f ~^3F_{2}$ &  $1s\,7f ~^3F_{3}$&  2.949E-07 &           &          &  5.254E-10 &            &   \\
$1s\,6g ~^3G_{3}$ &  $1s\,6g ~^3G_{4}$&  2.574E-07 &           &          &  5.099E-10 &            &   \\
$1s\,7f ~^1F_{3}$ &  $1s\,7f ~^3F_{4}$&  1.215E-07 &           &          &   2.81E-10 &            &   \\
$1s\,6g ~^1G_{4}$ &  $1s\,6g ~^3G_{5}$&  8.241E-08 &           &          &  2.703E-10 &            &   \\
$1s\,8f ~^3F_{2}$ &  $1s\,8f ~^3F_{3}$&  8.809E-08 &           &          &  3.536E-10 &            &   \\
$1s\,6h ~^3H_{4}$ &  $1s\,6h ~^3H_{5}$&  6.838E-08 &           &          &  3.363E-10 &            &   \\
$1s\,7g ~^3G_{3}$ &  $1s\,7g ~^3G_{4}$&  6.358E-08 &           &          &  3.177E-10 &            &   \\
$1s\,8f ~^1F_{3}$ &  $1s\,8f ~^3F_{4}$&  3.691E-08 &           &          &   1.87E-10 &            &   \\
$1s\,6h ~^1H_{5}$ &  $1s\,6h ~^3H_{6}$&  2.669E-08 &           &          &  1.968E-10 &            &   \\
$1s\,7g ~^1G_{4}$ &  $1s\,7g ~^3G_{5}$&  2.060E-08 &           &          &  1.701E-10 &            &   \\
$1s\,8g ~^3G_{3}$ &  $1s\,8g ~^3G_{4}$&  1.887E-08 &           &          &  2.102E-10 &            &   \\
$1s\,7h ~^3H_{4}$ &  $1s\,7h ~^3H_{5}$&  1.668E-08 &           &          &  2.067E-10 &            &   \\
$1s\,4d ~^3D_{1}$ &  $1s\,4d ~^3D_{2}$&  1.774E-08 &           &          &   2.22E-10 &            &   \\
$1s\,7h ~^1H_{5}$ &  $1s\,7h ~^3H_{6}$&  6.583E-09 &           &          &  1.224E-10 &            &   \\
$1s\,8g ~^1G_{4}$ &  $1s\,8g ~^3G_{5}$&  6.045E-09 &           &          &  1.111E-10 &            &   \\
$1s\,6d ~^3D_{2}$ &  $1s\,6d ~^3D_{1}$&  7.299E-09 &           &          &   3.27E-10 &            &   \\
$1s\,5d ~^3D_{2}$ &  $1s\,5d ~^3D_{1}$&  6.271E-09 &           &          &  3.111E-10 &            &   \\
$1s\,7i ~^3I_{5}$ &  $1s\,7i ~^3I_{6}$&  5.589E-09 &           &          &  1.452E-10 &            &   \\
$1s\,8h ~^3H_{4}$ &  $1s\,8h ~^3H_{5}$&  4.997E-09 &           &          &   1.38E-10 &            &   \\
$1s\,7d ~^3D_{2}$ &  $1s\,7d ~^3D_{1}$&  3.669E-09 &           &          &    2.6E-10 &            &   \\
$1s\,8d ~^3D_{2}$ &  $1s\,8d ~^3D_{1}$&  1.586E-09 &           &          &  1.956E-10 &            &   \\
\bottomrule
\end{longtable} 
\end{document}
