# Supplementary material for: Comprehensive calculations of energy levels, radiative transition parameters, hyperfine structure constants A$_J$-B$_J$, Land\'e g$_J$ factors and isotope shifts for Sc XX
Source: arXiv:2202.03112 source file (2022-02-07)
Supplement: Supplementary file 2 [file Table2.tex]

\documentclass[10pt]{article}
\usepackage{lscape}
\usepackage{booktabs}
\usepackage{longtable}
\usepackage{subfloat}
\textwidth = 15truecm
\textheight = 24 truecm
\hoffset = -4 truecm
\voffset = -2 truecm
\begin{document}
\caption{Table 2. Present radiative parameters for electric dipole  E1 transitions and their comparison with the results from Si et al. [32], Massacrier and Artru [36] and the NIST database [41]. } 
%Transition rate A and oscillator strength are tabulated here. Unit of A is $s^{-1}$ and f is a dimension less quantity}
% [inline block 0: 1 envs, 216160 chars -> data_tex | \begin{longtable}{lllllllll} \toprule...]

\end{document}
