# Supplementary material for: Comprehensive calculations of energy levels, radiative transition parameters, hyperfine structure constants A$_J$-B$_J$, Land\'e g$_J$ factors and isotope shifts for Sc XX
Source: arXiv:2202.03112 source file (2022-02-07)
Supplement: Supplementary file 4 [file Table5.tex]

\documentclass[10pt]{article}
\usepackage{booktabs}
\usepackage{longtable}
\usepackage{subfloat}
\usepackage{bm}
\textwidth = 15truecm
\textheight = 24 truecm
\hoffset = -3 truecm
\voffset = -2 truecm
\begin{document}
\caption{Table 5. Present radiative parameters for magnetic quadrupole M2 transitions and their comparison with the results from Si et al. [32] and the NIST database [41].}
% [inline block 0: 1 envs, 51687 chars -> data_tex | \begin{longtable}{lllllllll} \toprule...]

\end{document}
