# Supplementary material for: Comprehensive calculations of energy levels, radiative transition parameters, hyperfine structure constants A$_J$-B$_J$, Land\'e g$_J$ factors and isotope shifts for Sc XX
Source: arXiv:2202.03112 source file (2022-02-07)
Supplement: Supplementary file 5 [file Table6.tex]

\documentclass[10pt]{article}
\usepackage{booktabs}
\usepackage{longtable}
\usepackage{subfloat}
\textwidth = 15truecm
\textheight = 24 truecm
\hoffset = -2 truecm
\voffset = -2 truecm
\begin{document}
\caption{Table 6. Present results for lifetime of all the considered states and their comparison with the values from Si et al.[32]} 
\begin{longtable}{llll}
\toprule
     Level &      Our Work &      Si et al. [32] \\
\midrule
$1s\, 2s ~^3S_{ 1}$ & 4.9409E-08 & 4.3150E-08 \\
$1s\, 2p ~^3P_{ 0}$ & 3.8700E-09 & 3.8640E-09 \\
$1s\, 2p ~^3P_{ 1}$ & 1.3466E-13 & 1.3430E-13 \\
$1s\, 2s ~^1S_{ 0}$ & 5.7397E-04 & 6.6140E-04          \\
$1s\, 2p ~^3P_{ 2}$ & 5.9055E-10 & 5.9020E-10  \\
$1s\, 2p ~^1P_{ 1}$ & 5.0122E-15 & 5.0140E-15 \\
$1s\, 3s ~^3S_{ 1}$ & 8.1341E-13 & 8.1220E-13  \\
$1s\, 3p ~^3P_{ 0}$ & 2.7533E-13 & 2.7510E-13              \\
$1s\, 3s ~^1S_{ 0}$ & 8.5216E-13 & 8.5290E-13  \\
$1s\, 3p ~^3P_{ 1}$ & 1.7001E-13 & 1.6970E-13  \\
$1s\, 3p ~^3P_{ 2}$ & 2.8068E-13 & 2.8050E-13              \\
$1s\, 3d ~^3D_{ 2}$ & 9.5153E-14 & 9.4960E-14              \\
$1s\, 3d ~^3D_{ 1}$ & 9.4567E-14 & 9.4570E-14              \\
$1s\, 3d ~^3D_{ 3}$ & 9.5266E-14 & 9.5260E-14              \\
$1s\, 3p ~^1P_{ 1}$ & 1.7300E-14 & 1.7320E-14  \\
$1s\, 3d ~^1D_{ 2}$ & 9.6923E-14 & 9.6440E-14               \\
$1s\, 4s ~^3S_{ 1}$ & 1.1901E-12 & 1.1850E-12  \\
$1s\, 4p ~^3P_{ 0}$ & 4.6978E-13 & 4.6880E-13   \\
$1s\, 4s ~^1S_{ 0}$ & 1.2301E-12 & 1.2370E-12  \\
$1s\, 4p ~^3P_{ 1}$ & 3.2417E-13 & 3.2350E-13 \\
$1s\, 4p ~^3P_{ 2}$ & 4.7727E-13 & 4.7630E-13              \\
$1s\, 4d ~^3D_{ 2}$ & 2.2138E-13 & 2.2080E-13               \\
$1s\, 4d ~^3D_{ 1}$ & 2.1974E-13 & 2.1970E-13               \\
$1s\, 4d ~^3D_{ 3}$ & 2.2152E-13 & 2.2140E-13               \\
$1s\, 4p ~^1P_{ 1}$ & 4.1082E-14 & 4.1230E-14  \\
$1s\, 4f ~^3F_{ 3}$ & 4.5193E-13 & 4.5120E-13               \\
$1s\, 4d ~^1D_{ 2}$ & 2.2657E-13 & 2.2520E-13              \\
$1s\, 4f ~^3F_{ 2}$ & 4.5193E-13 & 4.5120E-13               \\
$1s\, 4f ~^3F_{ 4}$ & 4.5299E-13 & 4.5220E-13              \\
$1s\, 4f ~^1F_{ 3}$ & 4.5326E-13 & 4.5250E-13              \\
$1s\, 5s ~^3S_{ 1}$ & 1.8786E-12 & 1.8680E-12  \\
$1s\, 5p ~^3P_{ 0}$ & 8.0132E-13 & 7.9990E-13               \\
$1s\, 5s ~^1S_{ 0}$ & 1.9138E-12 & 1.9310E-12  \\
$1s\, 5p ~^3P_{ 1}$ & 5.7483E-13 & 5.7410E-13 \\
$1s\, 5p ~^3P_{ 2}$ & 8.1282E-13 & 8.1120E-13               \\
$1s\, 5d ~^3D_{ 1}$ & 4.2252E-13 & 4.2270E-13      \\
$1s\, 5d ~^3D_{ 2}$ & 4.2583E-13 & 4.2490E-13      \\
$1s\, 5d ~^3D_{ 3}$ & 4.2613E-13 & 4.2620E-13              \\
$1s\, 5p ~^1P_{ 1}$ & 7.9939E-14 & 8.0550E-14  \\
$1s\, 5f ~^3F_{ 3}$ & 8.7390E-13 & 8.7190E-13  \\
$1s\, 5d ~^1D_{ 2}$ & 4.3651E-13 & 4.3350E-13    \\
$1s\, 5f ~^3F_{ 2}$ & 8.7373E-13 & 8.7180E-13   \\
$1s\, 5f ~^3F_{ 4}$ & 8.7594E-13 & 8.7410E-13    \\
$1s\, 5g ~^3G_{ 4}$ & 1.4668E-12 & 1.4650E-12  \\
$1s\, 5g ~^3G_{ 3}$ & 1.4670E-12 & 1.4660E-12   \\
$1s\, 5f ~^1F_{ 3}$ & 8.7661E-13 & 8.7490E-13      \\
$1s\, 5g ~^3G_{ 5}$ & 1.4685E-12 & 1.4670E-12    \\
$1s\, 5g ~^1G_{ 4}$ & 1.4687E-12 & 1.4670E-12     \\
$1s\, 6s ~^3S_{ 1}$ & 2.8894E-12 & 2.9370E-12              \\
$1s\, 6p ~^3P_{ 0}$ & 1.2888E-12 & 1.3050E-12               \\
$1s\, 6s ~^1S_{ 0}$ & 2.8846E-12 & 2.8360E-12               \\
$1s\, 6p ~^3P_{ 1}$ & 9.4197E-13 & 9.5020E-13              \\
$1s\, 6p ~^3P_{ 2}$ & 1.3064E-12 & 1.3220E-12               \\
$1s\, 6d ~^3D_{ 1}$ & 7.2175E-13 & 7.2780E-13               \\
$1s\, 6d ~^3D_{ 2}$ & 7.2737E-13 & 7.2840E-13               \\
$1s\, 6d ~^3D_{ 3}$ & 7.2818E-13 & 7.3440E-13               \\
$1s\, 6p ~^1P_{ 1}$ & 1.3721E-13 & 1.3880E-13 &              \\
$1s\, 6f ~^3F_{ 3}$ & 1.4939E-12 & 1.4900E-12 &              \\
$1s\, 6d ~^1D_{ 2}$ & 7.4559E-13 & 7.3640E-13 &              \\
$1s\, 6f ~^3F_{ 2}$ & 1.4934E-12 & 1.4900E-12 &              \\
$1s\, 6f ~^3F_{ 4}$ & 1.4975E-12 & 1.4940E-12 &              \\
$1s\, 6g ~^3G_{ 4}$ & 2.5171E-12 & 2.5140E-12 &              \\
$1s\, 6g ~^3G_{ 3}$ & 2.5174E-12 & 2.5140E-12 &              \\
$1s\, 6f ~^1F_{ 3}$ & 1.4986E-12 & 1.4950E-12 &              \\
$1s\, 6g ~^3G_{ 5}$ & 2.5202E-12 & 2.5170E-12 &              \\
$1s\, 6h ~^3H_{ 5}$ & 3.7955E-12 & 3.7930E-12 &              \\
$1s\, 6h ~^3H_{ 4}$ & 3.7958E-12 & 3.7940E-12 &              \\
$1s\, 6g ~^1G_{ 4}$ & 2.5204E-12 & 2.5180E-12 &              \\
$1s\, 6h ~^3H_{ 6}$ & 3.7979E-12 & 3.7960E-12 &              \\
$1s\, 6h ~^1H_{ 5}$ & 3.7981E-12 & 3.7960E-12 &              \\
$1s\, 7s ~^3S_{ 1}$ & 4.2856E-12 &              &              \\
$1s\, 7p ~^3P_{ 0}$ & 1.9635E-12 &              &              \\
$1s\, 7s ~^1S_{ 0}$ & 4.1341E-12 &              &              \\
$1s\, 7p ~^3P_{ 1}$ & 1.4487E-12 &              &              \\
$1s\, 7p ~^3P_{ 2}$ & 1.9899E-12 &              &              \\
$1s\, 7d ~^3D_{ 1}$ & 1.1368E-12 &              &              \\
$1s\, 7d ~^3D_{ 2}$ & 1.1450E-12 &              &              \\
$1s\, 7d ~^3D_{ 3}$ & 1.1474E-12 &              &              \\
$1s\, 7p ~^1P_{ 1}$ & 2.1564E-13 &              &              \\
$1s\, 7f ~^3F_{ 3}$ & 2.3497E-12 &              &              \\
$1s\, 7d ~^1D_{ 2}$ & 1.1716E-12 &              &              \\
$1s\, 7f ~^3F_{ 2}$ & 2.3488E-12 &              &              \\
$1s\, 7f ~^3F_{ 4}$ & 2.3558E-12 &              &              \\
$1s\, 7g ~^3G_{ 4}$ & 3.9637E-12 &              &              \\
$1s\, 7g ~^3G_{ 3}$ & 3.9639E-12 &              &              \\
$1s\, 7f ~^1F_{ 3}$ & 2.3565E-12 &              &              \\
$1s\, 7g ~^3G_{ 5}$ & 3.9687E-12 &              &              \\
$1s\, 7h ~^3H_{ 5}$ & 5.9964E-12 &              &              \\
$1s\, 7h ~^3H_{ 4}$ & 5.9967E-12 &              &              \\
$1s\, 7g ~^1G_{ 4}$ & 3.9688E-12 &              &              \\
$1s\, 7h ~^3H_{ 6}$ & 6.0003E-12 &              &              \\
$1s\, 7i ~^3I_{ 6}$ & 8.4296E-12 &              &              \\
$1s\, 7i ~^3I_{ 5}$ & 8.4299E-12 &              &              \\
$1s\, 7h ~^1H_{ 5}$ & 6.0005E-12 &              &              \\
$1s\, 7i ~^3I_{ 7}$ & 8.4327E-12 &              &              \\
$1s\, 7i ~^1I_{ 6}$ & 8.4329E-12 &              &              \\
$1s\, 8s ~^3S_{ 1}$ & 6.1887E-12 &              &              \\
$1s\, 8p ~^3P_{ 0}$ & 2.8700E-12 &              &              \\
$1s\, 8s ~^1S_{ 0}$ & 5.5201E-12 &              &              \\
$1s\, 8p ~^3P_{ 1}$ & 2.1234E-12 &              &              \\
$1s\, 8p ~^3P_{ 2}$ & 2.9111E-12 &              &              \\
$1s\, 8d ~^3D_{ 1}$ & 1.6886E-12 &              &              \\
$1s\, 8d ~^3D_{ 2}$ & 1.6979E-12 &              &              \\
$1s\, 8d ~^3D_{ 3}$ & 1.7060E-12 &              &              \\
$1s\, 8p ~^1P_{ 1}$ & 3.1531E-13 &              &              \\
$1s\, 8f ~^3F_{ 3}$ & 3.4791E-12 &              &              \\
$1s\, 8d ~^1D_{ 2}$ & 1.7276E-12 &              &              \\
$1s\, 8f ~^3F_{ 2}$ & 3.4778E-12 &              &              \\
$1s\, 8f ~^3F_{ 4}$ & 3.4908E-12 &              &              \\
$1s\, 8g ~^3G_{ 4}$ & 5.8692E-12 &              &              \\
$1s\, 8f ~^1F_{ 3}$ & 3.4863E-12 &              &              \\
$1s\, 8g ~^3G_{ 3}$ & 5.8681E-12 &              &              \\
$1s\, 8g ~^3G_{ 5}$ & 5.8766E-12 &              &              \\
$1s\, 8h ~^3H_{ 5}$ & 8.8911E-12 &              &              \\
$1s\, 8h ~^3H_{ 4}$ & 8.8909E-12 &              &              \\
$1s\, 8g ~^1G_{ 4}$ & 5.8757E-12 &              &              \\
$1s\, 8h ~^3H_{ 6}$ & 8.8970E-12 &              &              \\
$1s\, 8i ~^3I_{ 6}$ & 1.2533E-11 &              &              \\
$1s\, 8i ~^3I_{ 5}$ & 1.2534E-11 &              &              \\
$1s\, 8h ~^1H_{ 5}$ & 8.8968E-12 &              &              \\
$1s\, 8i ~^3I_{ 7}$ & 1.2538E-11 &              &              \\
$1s\, 8k ~^3K_{ 7}$ & 1.6766E-11 &              &              \\
$1s\, 8i ~^1I_{ 6}$ & 1.2538E-11 &              &              \\
$1s\, 8k ~^3K_{ 6}$ & 1.6766E-11 &              &              \\
$1s\, 8k ~^3K_{ 8}$ & 1.6770E-11 &              &              \\
$1s\, 8k ~^1K_{ 7}$ & 1.6770E-11 &              &              \\
\bottomrule
\end{longtable}
\end{document}
