# Supplementary material for: Comprehensive calculations of energy levels, radiative transition parameters, hyperfine structure constants A$_J$-B$_J$, Land\'e g$_J$ factors and isotope shifts for Sc XX
Source: arXiv:2202.03112 source file (2022-02-07)
Supplement: Supplementary file 6 [file Table7.tex]

\documentclass[10pt]{article}
\usepackage{longtable}
\begin{document}

\caption{Table 7. Present results for hyperfine interaction constants A$_J$ and B$_J$ and Landé $g_J$ factors and their comparison with the corresponding values reported by Singh, et al. [20].}
\begin{longtable}{lrrrrr} \hline
State & A$_J$(MHz) & B$_J$(MHz) & 
$g_J$ & A$_J$(MHz) [20] & B$_J$(MHz) [20]  \\ \hline
 $1s\,2s~^3S_{   1}$ &     -1.847E+06 &     2.134E-01 &   1.990303 & -1.847E+06 &    2.098E-01 \\
 $1s\,2p~^3P_{   1}$ &     -1.278E+06 &     3.365E+03 &   1.474227 & -1.278E+06 &    3.355E+03\\
 $1s\,2p~^3P_{   2}$ &     -8.423E+05 &    -7.355E+03 &   1.493891 &    -8.423E+05 &    -7.333E+03 \\
 $1s\,2p~^1P_{   1}$ &      3.633E+05 &    -6.473E+03 &   1.016458  &  3.629E+05 &    -6.499E+03\\
 $1s\,3s~^3S_{   1}$ &     -1.711E+06 &     8.881E-02 &   1.991322 \\
 $1s\,3p~^3P_{   1}$ &     -1.267E+06 &     9.758E+02 &   1.473025 \\
 $1s\,3p~^3P_{   2}$ &     -8.317E+05 &    -2.173E+03 &   1.495104 \\
 $1s\,3d~^3D_{   2}$ &     -8.131E+05 &    -3.824E+02 &   1.112794 \\
 $1s\,3d~^3D_{   1}$ &      8.219E+05 &    -2.066E+02 &   0.502356 \\
 $1s\,3d~^3D_{   3}$ &     -5.528E+05 &    -5.830E+02 &   1.329693 \\
 $1s\,3p~^1P_{   1}$ &      4.138E+05 &    -1.928E+03 &   1.020652 \\
 $1s\,3d~^1D_{   2}$ &      5.323E+05 &    -4.970E+02 &   1.050190 \\
 $1s\,4s~^3S_{   1}$ &     -1.678E+06 &     4.149E-02 &   1.991675 \\
 $1s\,4p~^3P_{   1}$ &     -1.266E+06 &     4.078E+02 &   1.472583 \\
 $1s\,4p~^3P_{   2}$ &     -8.291E+05 &    -9.144E+02 &   1.495525 \\
 $1s\,4d~^3D_{   2}$ &     -8.011E+05 &    -1.585E+02 &   1.117745 \\
 $1s\,4d~^3D_{   1}$ &      8.249E+05 &    -8.739E+01 &   0.503049 \\
 $1s\,4d~^3D_{   3}$ &     -5.520E+05 &    -2.462E+02 &   1.330137 \\
 $1s\,4p~^1P_{   1}$ &      4.283E+05 &    -8.159E+02 &   1.022139 \\
 $1s\,4f~^3F_{   3}$ &     -5.518E+05 &    -8.739E+01 &   1.044266 \\
 $1s\,4d~^1D_{   2}$ &      5.232E+05 &    -2.135E+02 &   1.046276 \\
 $1s\,4f~^3F_{   2}$ &      5.508E+05 &    -6.986E+01 &   0.668492 \\
 $1s\,4f~^3F_{   4}$ &     -4.138E+05 &    -1.015E+02 &   1.247439 \\
 $1s\,4f~^1F_{   3}$ &      4.132E+05 &    -9.058E+01 &   1.037079 \\
 $1s\,5s~^3S_{   1}$ &     -1.666E+06 &     2.214E-02 &   1.991838 \\
 $1s\,5p~^3P_{   1}$ &     -1.267E+06 &     2.075E+02 &   1.472402 \\
 $1s\,5p~^3P_{   2}$ &     -8.281E+05 &    -4.670E+02 &   1.495720 \\
 $1s\,5d~^3D_{   1}$ &      8.260E+05 &    -4.479E+01 &   0.503369 \\
 $1s\,5d~^3D_{   2}$ &     -7.955E+05 &    -8.060E+01 &   1.119754 \\
 $1s\,5d~^3D_{   3}$ &     -5.517E+05 &    -1.261E+02 &   1.330343 \\
 $1s\,5p~^1P_{   1}$ &      4.340E+05 &    -4.195E+02 &   1.022803 \\
 $1s\,5f~^3F_{   3}$ &     -5.516E+05 &    -4.477E+01 &   1.044685 \\
 $1s\,5d~^1D_{   2}$ &      5.187E+05 &    -1.101E+02 &   1.044746 \\
 $1s\,5f~^3F_{   2}$ &      5.511E+05 &    -3.582E+01 &   0.668780 \\
 $1s\,5f~^3F_{   4}$ &     -4.137E+05 &    -5.202E+01 &   1.247652 \\
 $1s\,5g~^3G_{   4}$ &     -4.136E+05 &    -2.446E+01 &   1.025186 \\
 $1s\,5g~^3G_{   3}$ &      4.134E+05 &    -2.182E+01 &   0.751481 \\
 $1s\,5f~^1F_{   3}$ &      4.134E+05 &    -4.645E+01 &   1.037139 \\
 $1s\,5g~^3G_{   5}$ &     -3.309E+05 &    -2.662E+01 &   1.198038 \\
 $1s\,5g~^1G_{   4}$ &      3.307E+05 &    -2.482E+01 &   1.023568 \\
 $1s\,6s~^3S_{   1}$ &     -1.661E+06 &     1.304E-02 &   1.991926 \\
 $1s\,6p~^3P_{   1}$ &     -1.267E+06 &     1.195E+02 &   1.472349 \\
 $1s\,6p~^3P_{   2}$ &     -8.277E+05 &    -2.695E+02 &   1.495825 \\
 $1s\,6d~^3D_{   1}$ &      8.264E+05 &    -2.593E+01 &   0.503543 \\
 $1s\,6d~^3D_{   2}$ &     -7.926E+05 &    -4.647E+01 &   1.120783 \\
 $1s\,6d~^3D_{   3}$ &     -5.516E+05 &    -7.297E+01 &   1.330455 \\
 $1s\,6p~^1P_{   1}$ &      4.364E+05 &    -2.443E+02 &   1.023118 \\
 $1s\,6f~^3F_{   3}$ &     -5.515E+05 &    -2.591E+01 &   1.044923 \\
 $1s\,6d~^1D_{   2}$ &      5.163E+05 &    -6.400E+01 &   1.043978 \\
 $1s\,6f~^3F_{   2}$ &      5.512E+05 &    -2.074E+01 &   0.668936 \\
 $1s\,6f~^3F_{   4}$ &     -4.136E+05 &    -3.012E+01 &   1.247768 \\
 $1s\,6g~^3G_{   4}$ &     -4.136E+05 &    -1.416E+01 &   1.025305 \\
 $1s\,6g~^3G_{   3}$ &      4.135E+05 &    -1.264E+01 &   0.751630 \\
 $1s\,6f~^1F_{   3}$ &      4.134E+05 &    -2.691E+01 &   1.037162 \\
 $1s\,6g~^3G_{   5}$ &     -3.309E+05 &    -1.541E+01 &   1.198156 \\
 $1s\,6h~^3H_{   5}$ &     -3.309E+05 &    -8.351 &   1.016202 \\
 $1s\,6h~^3H_{   4}$ &      3.308E+05 &    -7.791 &   0.801246 \\
 $1s\,6g~^1G_{   4}$ &      3.308E+05 &    -1.437E+01 &   1.023709 \\
 $1s\,6h~^3H_{   6}$ &     -2.757E+05 &    -8.821 &   1.165081 \\
 $1s\,6h~^1H_{   5}$ &      2.757E+05 &    -8.417 &   1.016277 \\
 $1s\,7s~^3S_{   1}$ &     -1.659E+06 &     8.249E-03 &   1.991980 \\
 $1s\,7p~^3P_{   1}$ &     -1.266E+06 &     7.487E+01 &   1.472375 \\
 $1s\,7p~^3P_{   2}$ &     -8.275E+05 &    -1.691E+02 &   1.495889 \\
 $1s\,7d~^3D_{   1}$ &      8.267E+05 &    -1.633E+01 &   0.503648 \\
 $1s\,7d~^3D_{   2}$ &     -7.909E+05 &    -2.920E+01 &   1.121387 \\
 $1s\,7d~^3D_{   3}$ &     -5.515E+05 &    -4.593E+01 &   1.330523 \\
 $1s\,7p~^1P_{   1}$ &      4.373E+05 &    -1.553E+02 &   1.023249 \\
 $1s\,7f~^3F_{   3}$ &     -5.515E+05 &    -1.632E+01 &   1.045070 \\
 $1s\,7d~^1D_{   2}$ &      5.147E+05 &    -4.042E+01 &   1.043532 \\
 $1s\,7f~^3F_{   2}$ &      5.513E+05 &    -1.307E+01 &   0.669030 \\
 $1s\,7f~^3F_{   4}$ &     -4.136E+05 &    -1.897E+01 &   1.247838 \\
 $1s\,7g~^3G_{   4}$ &     -4.136E+05 &    -8.922 &   1.025377 \\
 $1s\,7g~^3G_{   3}$ &      4.135E+05 &    -7.961 &   0.751720 \\
 $1s\,7f~^1F_{   3}$ &      4.135E+05 &    -1.696E+01 &   1.037173 \\
 $1s\,7g~^3G_{   5}$ &     -3.309E+05 &    -9.708 &   1.198228 \\
 $1s\,7h~^3H_{   5}$ &     -3.308E+05 &    -5.261 &   1.016274 \\
 $1s\,7h~^3H_{   4}$ &      3.308E+05 &    -4.908 &   0.801333 \\
 $1s\,7g~^1G_{   4}$ &      3.308E+05 &    -9.054 &   1.023795 \\
 $1s\,7h~^3H_{   6}$ &     -2.757E+05 &    -5.557 &   1.165154 \\
 $1s\,7i~^3I_{   6}$ &     -2.757E+05 &    -3.382 &   1.011225 \\
 $1s\,7i~^3I_{   5}$ &      2.757E+05 &    -3.228 &   0.834408 \\
 $1s\,7h~^1H_{   5}$ &      2.757E+05 &    -5.302 &   1.016362 \\
 $1s\,7i~^3I_{   7}$ &     -2.363E+05 &    -3.515 &   1.141529 \\
 $1s\,7i~^1I_{   6}$ &      2.363E+05 &    -3.398 &   1.011962 \\
 $1s\,8s~^3S_{   1}$ &     -1.657E+06 &     5.476E-03 &   1.992017 \\
 $1s\,8p~^3P_{   1}$ &     -1.265E+06 &     4.979E+01 &   1.472554 \\
 $1s\,8p~^3P_{   2}$ &     -8.273E+05 &    -1.125E+02 &   1.495932 \\
 $1s\,8d~^3D_{   1}$ &      8.268E+05 &    -1.094E+01 &   0.503714 \\
 $1s\,8d~^3D_{   2}$ &     -7.896E+05 &    -1.953E+01 &   1.121801 \\
 $1s\,8d~^3D_{   3}$ &     -5.515E+05 &    -3.075E+01 &   1.330567 \\
 $1s\,8p~^1P_{   1}$ &      4.364E+05 &    -1.061E+02 &   1.023172 \\
 $1s\,8f~^3F_{   3}$ &     -5.514E+05 &    -1.093E+01 &   1.045166 \\
 $1s\,8d~^1D_{   2}$ &      5.137E+05 &    -2.715E+01 &   1.043220 \\
 $1s\,8f~^3F_{   2}$ &      5.513E+05 &    -8.757 &   0.669090 \\
 $1s\,8f~^3F_{   4}$ &     -4.136E+05 &    -1.271E+01 &   1.247884 \\
 $1s\,8g~^3G_{   4}$ &     -4.136E+05 &    -5.978 &   1.025423 \\
 $1s\,8f~^1F_{   3}$ &      4.135E+05 &    -1.136E+01 &   1.037178 \\
 $1s\,8g~^3G_{   3}$ &      4.135E+05 &    -5.335 &   0.751778 \\
 $1s\,8g~^3G_{   5}$ &     -3.309E+05 &    -6.505 &   1.198274 \\
 $1s\,8h~^3H_{   5}$ &     -3.308E+05 &    -3.525 &   1.016320 \\
 $1s\,8h~^3H_{   4}$ &      3.308E+05 &    -3.289 &   0.801389 \\
 $1s\,8g~^1G_{   4}$ &      3.308E+05 &    -6.067 &   1.023850 \\
 $1s\,8h~^3H_{   6}$ &     -2.757E+05 &    -3.724 &   1.165201 \\
 $1s\,8i~^3I_{   6}$ &     -2.757E+05 &    -2.266 &   1.011272 \\
 $1s\,8i~^3I_{   5}$ &      2.757E+05 &    -2.163 &   0.834464 \\
 $1s\,8h~^1H_{   5}$ &      2.757E+05 &    -3.553 &   1.016418 \\
 $1s\,8i~^3I_{   7}$ &     -2.363E+05 &    -2.355 &   1.141577 \\
 $1s\,8k~^3K_{   7}$ &     -2.363E+05 &    -1.521 &   1.008190 \\
 $1s\,8i~^1I_{   6}$ &      2.363E+05 &    -2.277 &   1.012017 \\
 $1s\,8k~^3K_{   6}$ &      2.363E+05 &    -1.470 &   0.858088 \\
 $1s\,8k~^3K_{   8}$ &     -2.068E+05 &    -1.564 &   1.123859 \\
 $1s\,8k~^1K_{   7}$ &      2.068E+05 &    -1.525 &   1.009194 \\
\hline\\

\end{longtable}
\end{document}
