# Supplementary material for: Comprehensive calculations of energy levels, radiative transition parameters, hyperfine structure constants A$_J$-B$_J$, Land\'e g$_J$ factors and isotope shifts for Sc XX
Source: arXiv:2202.03112 source file (2022-02-07)
Supplement: Supplementary file 7 [file Table8.tex]

\documentclass[10pt]{article}
\usepackage{longtable}
\begin{document}
\caption{Table 8. Present results for isotope shift parameters; NMS  $\times 10^2$ a.u., SMS in a.u. and  FS $\times 10^2$ GHz/fm^2.   }
\begin{longtable}{llrr} \hline
State &  NMS & 
SMS & FS \\ \hline
 $1s^2 ~^1S_{   0}$ &   4.275456     &  2.787607     &     6.854646    \\
 $1s\,2s~^3S_{   1}$ &   2.719923     &  2.203885E-01 &     3.960736    \\
 $1s\,2p~^3P_{   0}$ &   2.710602     & -3.092462E+01 &     3.532167    \\
 $1s\,2p~^3P_{   1}$ &   2.710856     & -2.885961E+01 &     3.532787    \\
 $1s\,2s~^1S_{   0}$ &   2.710428     &  3.125876E-01 &     3.948157    \\
 $1s\,2p~^3P_{   2}$ &   2.709226     & -3.114092E+01 &     3.531048    \\
 $1s\,2p~^1P_{   1}$ &   2.703604     &  2.851542E+01 &     3.547489    \\
 $1s\,3s~^3S_{   1}$ &   2.431447     &  7.303088E-02 &     3.666331    \\
 $1s\,3p~^3P_{   0}$ &   2.428945     & -7.027844     &     3.541524    \\
 $1s\,3s~^1S_{   0}$ &   2.429365     &  1.075378E-01 &     3.664131    \\
 $1s\,3p~^3P_{   1}$ &   2.429004     & -6.502565     &     3.541677    \\
 $1s\,3p~^3P_{   2}$ &   2.428501     & -7.160304     &     3.541104    \\
 $1s\,3d~^3D_{   2}$ &   2.427316     & -3.683133E-03 &     3.544268    \\
 $1s\,3d~^3D_{   1}$ &   2.427243     &  2.183848E-02 &     3.544157    \\
 $1s\,3d~^3D_{   3}$ &   2.427077     &  1.724168E-02 &     3.544158    \\
 $1s\,3p~^1P_{   1}$ &   2.427110     &  6.708617     &     3.544721    \\
 $1s\,3d~^1D_{   2}$ &   2.427030     & -3.651629E-02 &     3.544421    \\
 $1s\,4s~^3S_{   1}$ &   2.331571     &  3.406517E-02 &     3.595477    \\
 $1s\,4p~^3P_{   0}$ &   2.330618     & -2.714603     &     3.543297    \\
 $1s\,4s~^1S_{   0}$ &   2.331283     &  5.014035E-02 &     3.595087    \\
 $1s\,4p~^3P_{   1}$ &   2.330640     & -2.503440     &     3.543357    \\
 $1s\,4p~^3P_{   2}$ &   2.330412     & -2.777038     &     3.543107    \\
 $1s\,4d~^3D_{   2}$ &   2.329988     &  2.148570E-03 &     3.544353    \\
 $1s\,4d~^3D_{   1}$ &   2.329961     &  1.435740E-02 &     3.544301    \\
 $1s\,4d~^3D_{   3}$ &   2.329876     &  1.240623E-02 &     3.544301    \\
 $1s\,4p~^1P_{   1}$ &   2.330100     &  2.628013     &     3.544481    \\
 $1s\,4f~^3F_{   3}$ &   2.329868     & -2.059344E-03 &     3.544433    \\
 $1s\,4d~^1D_{   2}$ &   2.329902     & -1.747462E-02 &     3.544442    \\
 $1s\,4f~^3F_{   2}$ &   2.329853     & -1.275235E-03 &     3.544431    \\
 $1s\,4f~^3F_{   4}$ &   2.329816     & -2.355274E-03 &     3.544431    \\
 $1s\,4f~^1F_{   3}$ &   2.329806     & -2.133123E-03 &     3.544434    \\
 $1s\,5s~^3S_{   1}$ &   2.285600     &  1.909353E-02 &     3.570417    \\
 $1s\,5p~^3P_{   0}$ &   2.285184     & -1.333278     &     3.543874    \\
 $1s\,5s~^1S_{   0}$ &   2.285997     &  2.795237E-02 &     3.570524    \\
 $1s\,5p~^3P_{   1}$ &   2.285193     & -1.227390     &     3.543904    \\
 $1s\,5p~^3P_{   2}$ &   2.285059     & -1.366398     &     3.543774    \\
 $1s\,5d~^3D_{   1}$ &   2.284909     &  8.955058E-03 &     3.544370    \\
 $1s\,5d~^3D_{   2}$ &   2.284922     &  2.443255E-03 &     3.544397    \\
 $1s\,5d~^3D_{   3}$ &   2.284855     &  7.937232E-03 &     3.544370    \\
 $1s\,5p~^1P_{   1}$ &   2.285200     &  1.305566     &     3.544443    \\
 $1s\,5f~^3F_{   3}$ &   2.284860     & -1.060568E-03 &     3.544434    \\
 $1s\,5d~^1D_{   2}$ &   2.284905     & -8.940960E-03 &     3.544448    \\
 $1s\,5f~^3F_{   2}$ &   2.284856     & -5.887664E-04 &     3.544433    \\
 $1s\,5f~^3F_{   4}$ &   2.284833     & -1.147661E-03 &     3.544433    \\
 $1s\,5g~^3G_{   4}$ &   2.284841     & -1.989099E-04 &     3.544455    \\
 $1s\,5g~^3G_{   3}$ &   2.284837     & -4.388311E-05 &     3.544455    \\
 $1s\,5f~^1F_{   3}$ &   2.284832     & -1.119455E-03 &     3.544435    \\
 $1s\,5g~^3G_{   5}$ &   2.284826     & -3.668147E-04 &     3.544455    \\
 $1s\,5g~^1G_{   4}$ &   2.284822     & -2.143352E-04 &     3.544455    \\
 $1s\,6s~^3S_{   1}$ &   2.260712     &  1.203340E-02 &     3.559393    \\
 $1s\,6p~^3P_{   0}$ &   2.260529     & -7.531964E-01 &     3.544118    \\
 $1s\,6s~^1S_{   0}$ &   2.261461     &  1.753500E-02 &     3.559669    \\
 $1s\,6p~^3P_{   1}$ &   2.260533     & -6.925164E-01 &     3.544135    \\
 $1s\,6p~^3P_{   2}$ &   2.260437     & -7.724976E-01 &     3.544059    \\
 $1s\,6d~^3D_{   1}$ &   2.260434     &  5.962453E-03 &     3.544404    \\
 $1s\,6d~^3D_{   2}$ &   2.260441     &  2.115898E-03 &     3.544420    \\
 $1s\,6d~^3D_{   3}$ &   2.260395     &  5.358306E-03 &     3.544404    \\
 $1s\,6p~^1P_{   1}$ &   2.260836     &  7.468048E-01 &     3.544436    \\
 $1s\,6f~^3F_{   3}$ &   2.260405     & -4.638630E-04 &     3.544436    \\
 $1s\,6d~^1D_{   2}$ &   2.260454     & -4.884774E-03 &     3.544451    \\
 $1s\,6f~^3F_{   2}$ &   2.260406     & -1.657691E-04 &     3.544435    \\
 $1s\,6f~^3F_{   4}$ &   2.260389     & -4.968594E-04 &     3.544435    \\
 $1s\,6g~^3G_{   4}$ &   2.260397     & -9.618231E-05 &     3.544455    \\
 $1s\,6g~^3G_{   3}$ &   2.260396     & -4.323317E-06 &     3.544455    \\
 $1s\,6f~^1F_{   3}$ &   2.260392     & -5.047735E-04 &     3.544436    \\
 $1s\,6g~^3G_{   5}$ &   2.260388     & -1.960606E-04 &     3.544455    \\
 $1s\,6h~^3H_{   5}$ &   2.260383     & -3.971349E-05 &     3.544437    \\
 $1s\,6h~^3H_{   4}$ &   2.260381     &  2.529173E-05 &     3.544437    \\
 $1s\,6g~^1G_{   4}$ &   2.260388     & -1.068730E-04 &     3.544455    \\
 $1s\,6h~^3H_{   6}$ &   2.260377     & -1.038676E-04 &     3.544437    \\
 $1s\,6h~^1H_{   5}$ &   2.260375     & -3.884112E-05 &     3.544437    \\
 $1s\,7s~^3S_{   1}$ &   2.245719     &  8.283597E-03 &     3.553804    \\
 $1s\,7p~^3P_{   0}$ &   2.245662     & -4.664972E-01 &     3.544239    \\
 $1s\,7s~^1S_{   0}$ &   2.246767     &  1.205245E-02 &     3.554159    \\
 $1s\,7p~^3P_{   1}$ &   2.245663     & -4.284011E-01 &     3.544250    \\
 $1s\,7p~^3P_{   2}$ &   2.245580     & -4.784891E-01 &     3.544202    \\
 $1s\,7d~^3D_{   1}$ &   2.245677     &  4.270278E-03 &     3.544422    \\
 $1s\,7d~^3D_{   2}$ &   2.245680     &  1.816674E-03 &     3.544432    \\
 $1s\,7d~^3D_{   3}$ &   2.245643     &  3.879661E-03 &     3.544423    \\
 $1s\,7p~^1P_{   1}$ &   2.246208     &  4.701112E-01 &     3.544435    \\
 $1s\,7f~^3F_{   3}$ &   2.245658     & -9.652587E-05 &     3.544436    \\
 $1s\,7d~^1D_{   2}$ &   2.245711     & -2.744357E-03 &     3.544453    \\
 $1s\,7f~^3F_{   2}$ &   2.245662     &  1.023816E-04 &     3.544436    \\
 $1s\,7f~^3F_{   4}$ &   2.245648     & -1.135280E-04 &     3.544435    \\
 $1s\,7g~^3G_{   4}$ &   2.245656     &  2.572034E-05 &     3.544455    \\
 $1s\,7g~^3G_{   3}$ &   2.245657     &  8.491407E-05 &     3.544455    \\
 $1s\,7f~^1F_{   3}$ &   2.245653     & -1.246980E-04 &     3.544436    \\
 $1s\,7g~^3G_{   5}$ &   2.245651     & -3.627631E-05 &     3.544455    \\
 $1s\,7h~^3H_{   5}$ &   2.245645     & -6.802523E-07 &     3.544437    \\
 $1s\,7h~^3H_{   4}$ &   2.245645     &  4.072826E-05 &     3.544437    \\
 $1s\,7g~^1G_{   4}$ &   2.245652     &  2.153181E-05 &     3.544455    \\
 $1s\,7h~^3H_{   6}$ &   2.245641     & -4.107832E-05 &     3.544437    \\
 $1s\,7i~^3I_{   6}$ &   2.245647     & -3.388270E-05 &     3.544455    \\
 $1s\,7i~^3I_{   5}$ &   2.245647     & -6.939885E-06 &     3.544455    \\
 $1s\,7h~^1H_{   5}$ &   2.245641     &  3.058021E-07 &     3.544437    \\
 $1s\,7i~^3I_{   7}$ &   2.245645     & -6.587238E-05 &     3.544455    \\
 $1s\,7i~^1I_{   6}$ &   2.245644     & -3.909526E-05 &     3.544455    \\
 $1s\,8s~^3S_{   1}$ &   2.235915     &  6.217944E-03 &     3.550661    \\
 $1s\,8p~^3P_{   0}$ &   2.235965     & -3.079258E-01 &     3.544306    \\
 $1s\,8s~^1S_{   0}$ &   2.237581     &  9.110173E-03 &     3.551120    \\
 $1s\,8p~^3P_{   1}$ &   2.235963     & -2.823452E-01 &     3.544313    \\
 $1s\,8p~^3P_{   2}$ &   2.235869     & -3.155740E-01 &     3.544282    \\
 $1s\,8d~^3D_{   1}$ &   2.236098     &  3.354020E-03 &     3.544433    \\
 $1s\,8d~^3D_{   2}$ &   2.236099     &  1.693140E-03 &     3.544440    \\
 $1s\,8d~^3D_{   3}$ &   2.236062     &  3.080608E-03 &     3.544433    \\
 $1s\,8p~^1P_{   1}$ &   2.236942     &  3.193197E-01 &     3.544435    \\
 $1s\,8f~^3F_{   3}$ &   2.236086     &  2.040669E-04 &     3.544437    \\
 $1s\,8d~^1D_{   2}$ &   2.236155     & -1.430518E-03 &     3.544454    \\
 $1s\,8f~^3F_{   2}$ &   2.236095     &  3.440163E-04 &     3.544436    \\
 $1s\,8f~^3F_{   4}$ &   2.236080     &  1.911302E-04 &     3.544436    \\
 $1s\,8g~^3G_{   4}$ &   2.236088     &  2.045608E-04 &     3.544455    \\
 $1s\,8f~^1F_{   3}$ &   2.236088     &  1.844840E-04 &     3.544437    \\
 $1s\,8g~^3G_{   3}$ &   2.236092     &  2.469895E-04 &     3.544455    \\
 $1s\,8g~^3G_{   5}$ &   2.236085     &  1.595294E-04 &     3.544455    \\
 $1s\,8h~^3H_{   5}$ &   2.236079     &  1.178947E-04 &     3.544437    \\
 $1s\,8h~^3H_{   4}$ &   2.236081     &  1.471717E-04 &     3.544437    \\
 $1s\,8g~^1G_{   4}$ &   2.236088     &  2.007563E-04 &     3.544455    \\
 $1s\,8h~^3H_{   6}$ &   2.236077     &  8.965536E-05 &     3.544437    \\
 $1s\,8i~^3I_{   6}$ &   2.236083     &  3.234277E-05 &     3.544455    \\
 $1s\,8i~^3I_{   5}$ &   2.236083     &  5.086809E-05 &     3.544455    \\
 $1s\,8h~^1H_{   5}$ &   2.236078     &  1.188620E-04 &     3.544437    \\
 $1s\,8i~^3I_{   7}$ &   2.236081     &  1.317226E-05 &     3.544455    \\
 $1s\,8k~^3K_{   7}$ &   2.236074     & -6.251764E-04 &     3.544437    \\
 $1s\,8i~^1I_{   6}$ &   2.236081     &  3.180782E-05 &     3.544455    \\
 $1s\,8k~^3K_{   6}$ &   2.236074     & -6.175554E-04 &     3.544437    \\
 $1s\,8k~^3K_{   8}$ &   2.236073     & -6.328979E-04 &     3.544437    \\
 $1s\,8k~^1K_{   7}$ &   2.236073     & -6.251633E-04 &     3.544437    \\
\hline\\
\end{longtable}
\end{document}
